# Supplementary material for: HarmonicNeRF: Geometry-Informed Synthetic View Augmentation for 3D Scene Reconstruction in Driving Scenarios
Source: arXiv:2310.05483 source file (2024-07-25)
Supplement: Supplementary file 1 [file mesh.tex]

\begin{figure}[!b]
    \centering
    \rotatebox[origin=C]{90}{\parbox{20mm}{\centering \small Chair \\ (Blender)}} 
  \mpage{0.20}{\includegraphics[width=\linewidth]{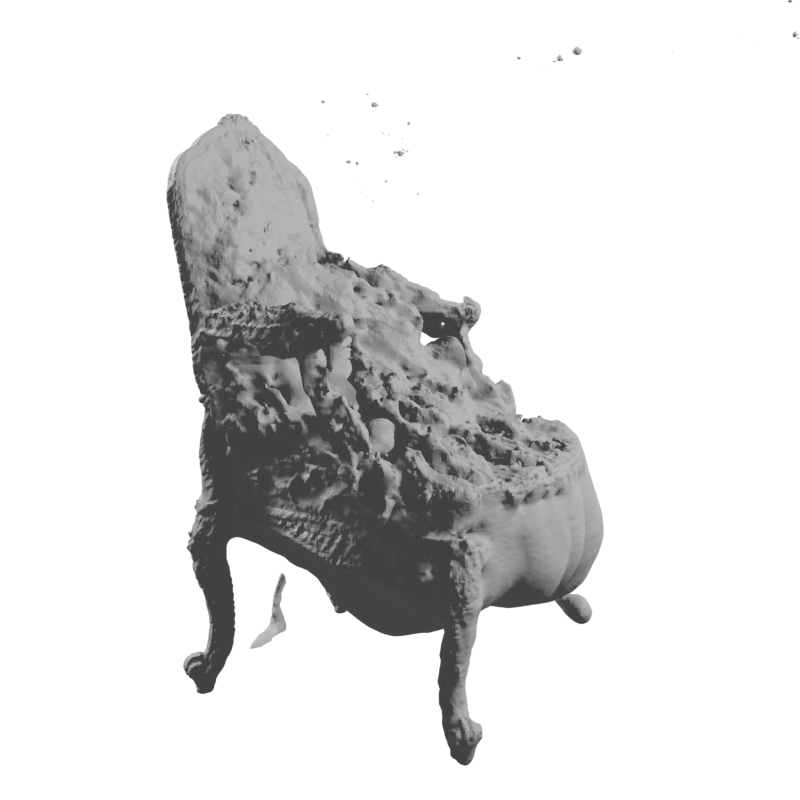}}
  \mpage{0.20}{\includegraphics[width=\linewidth]{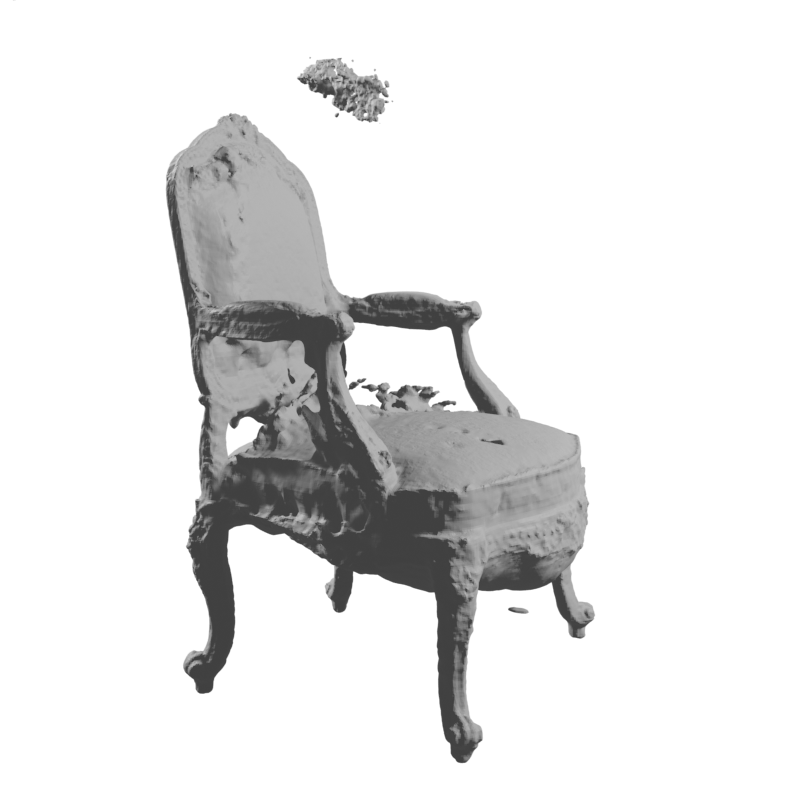}}
  \mpage{0.20}{\includegraphics[width=\linewidth]{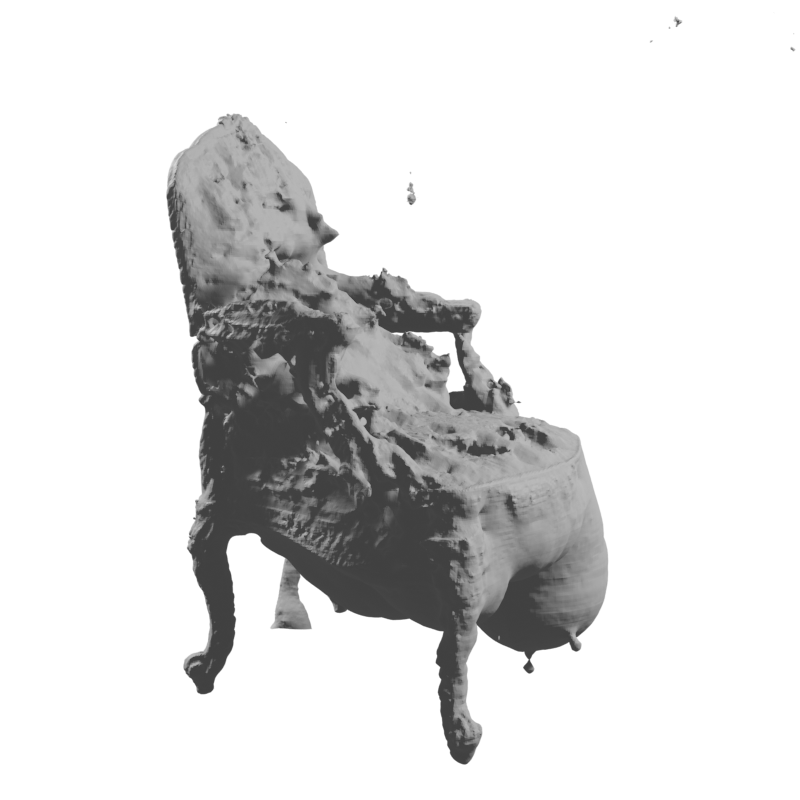}}
  \mpage{0.20}{\includegraphics[width=\linewidth]{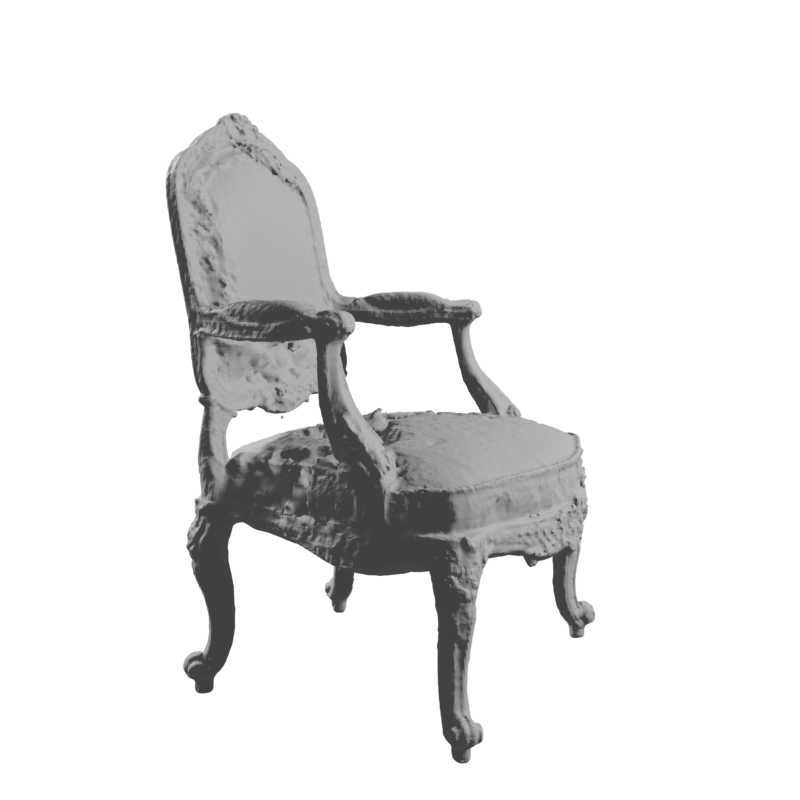}}
  \\
  \rotatebox[origin=C]{90}{\parbox{20mm}{\centering \small Ficus \\ (Blender)}} 
  \mpage{0.20}{\includegraphics[width=\linewidth]{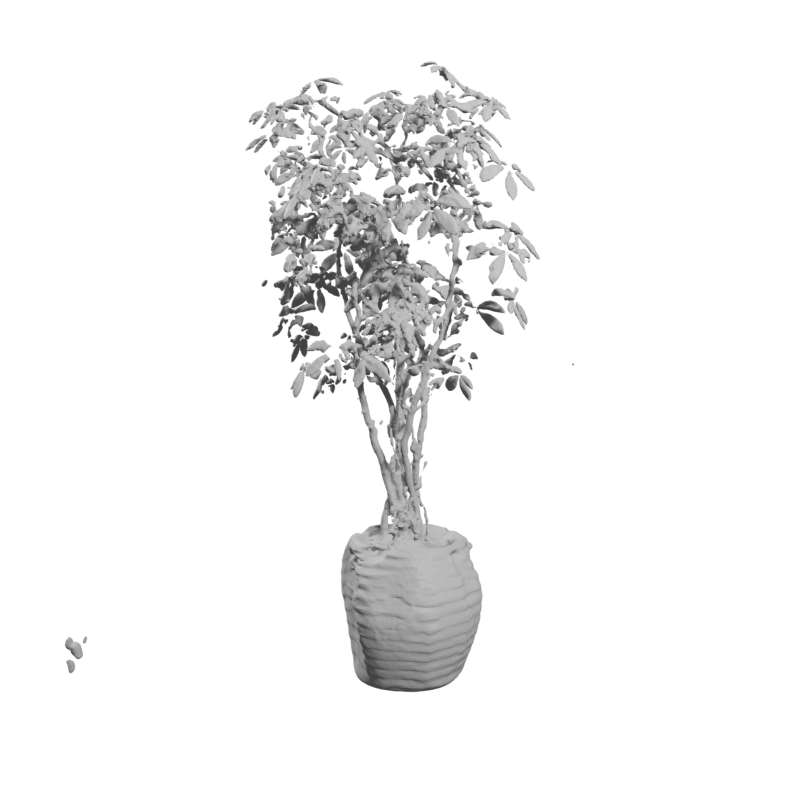}}
  \mpage{0.20}{\includegraphics[width=\linewidth]{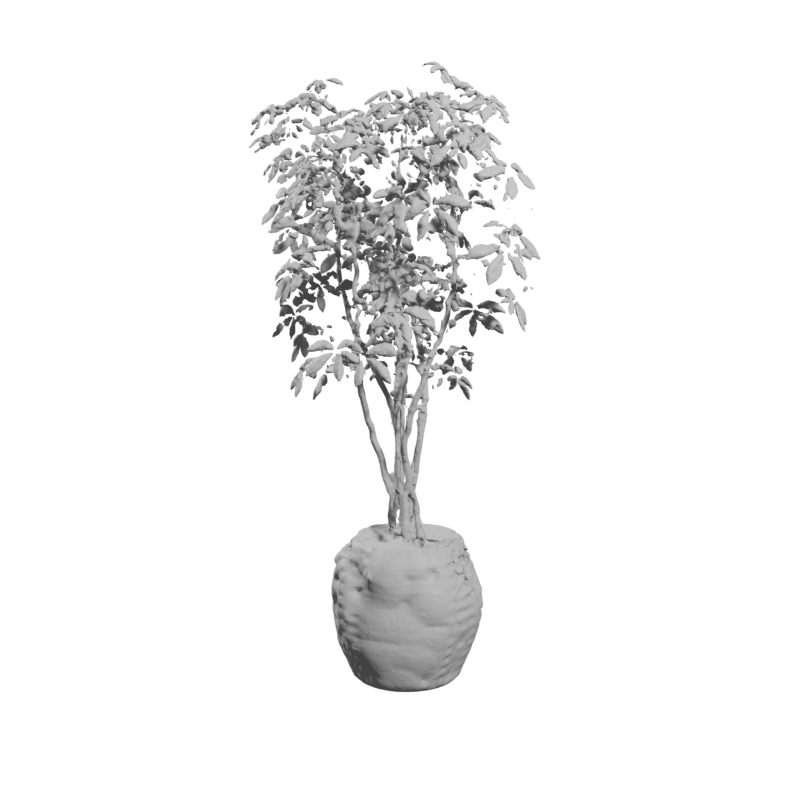}}
  \mpage{0.20}{\includegraphics[width=\linewidth]{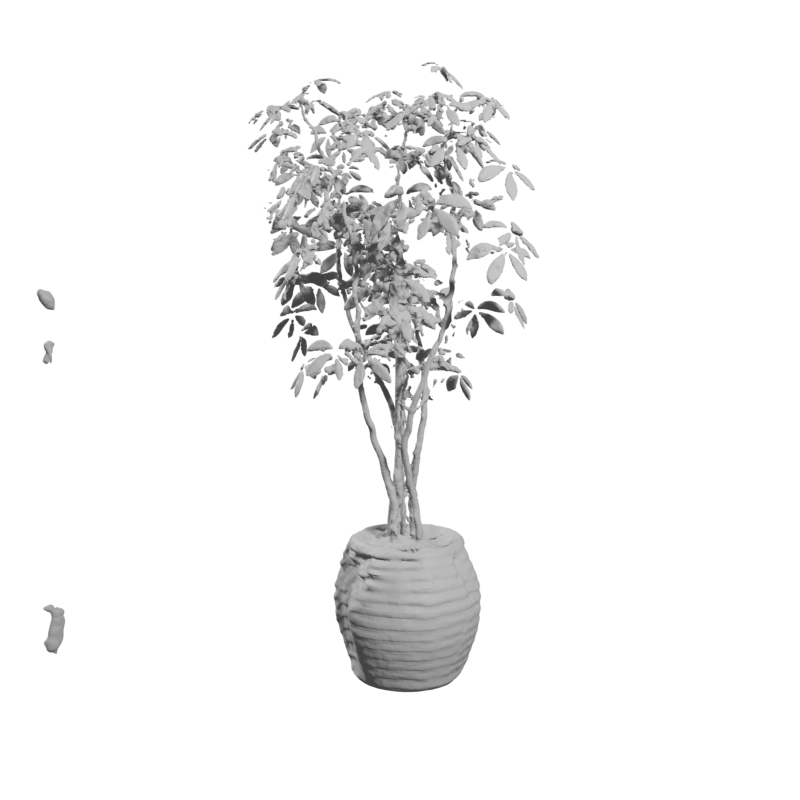}}
  \mpage{0.20}{\includegraphics[width=\linewidth]{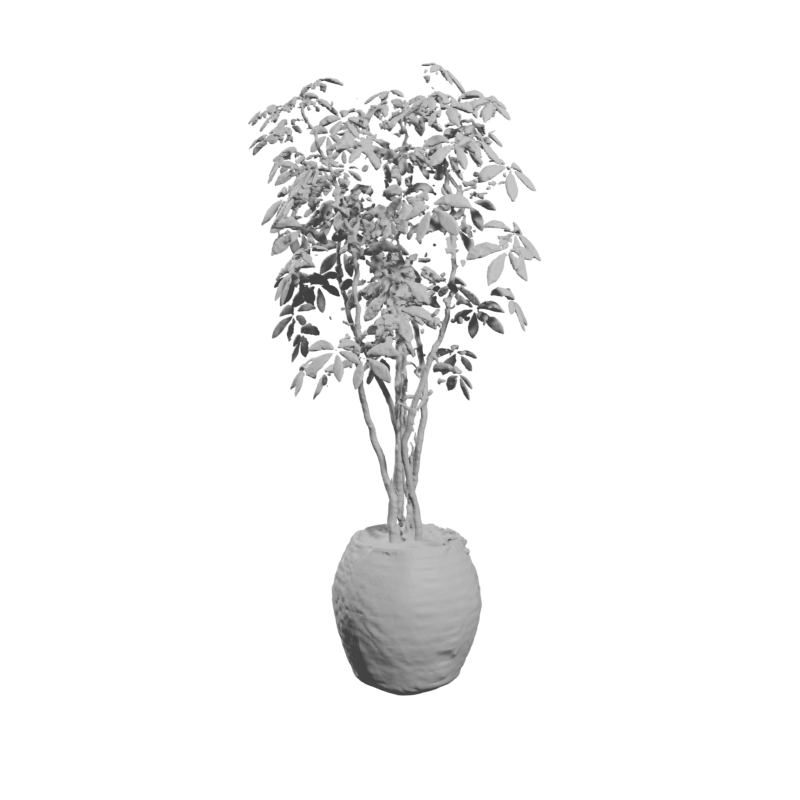}}
 \\
   \rotatebox[origin=C]{90}{\parbox{20mm}{\centering \small Lego \\ (Blender)}} 
  \mpage{0.20}{\includegraphics[width=\linewidth]{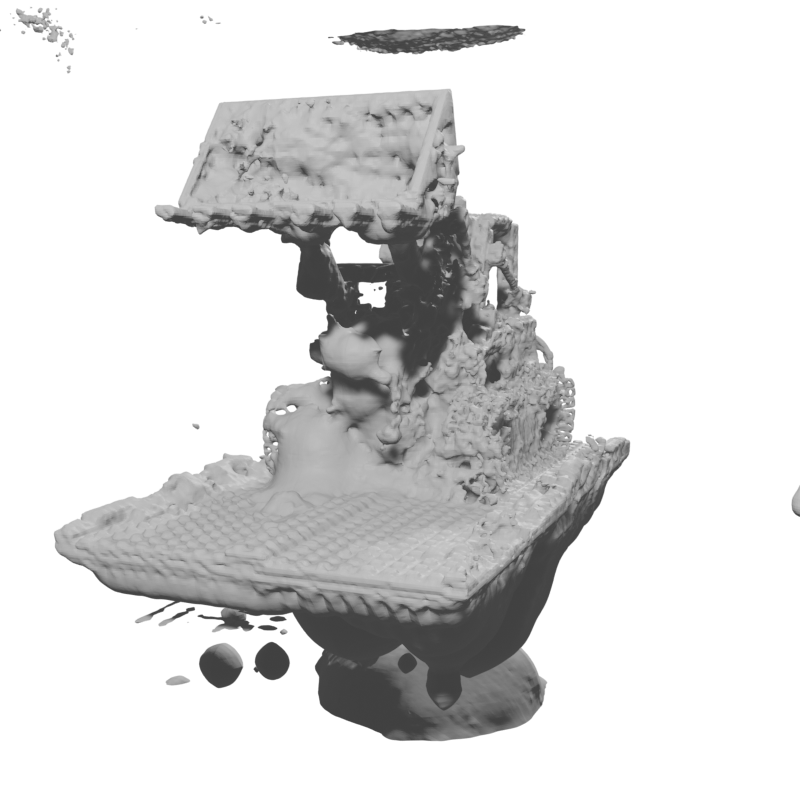}}
  \mpage{0.20}{\includegraphics[width=\linewidth]{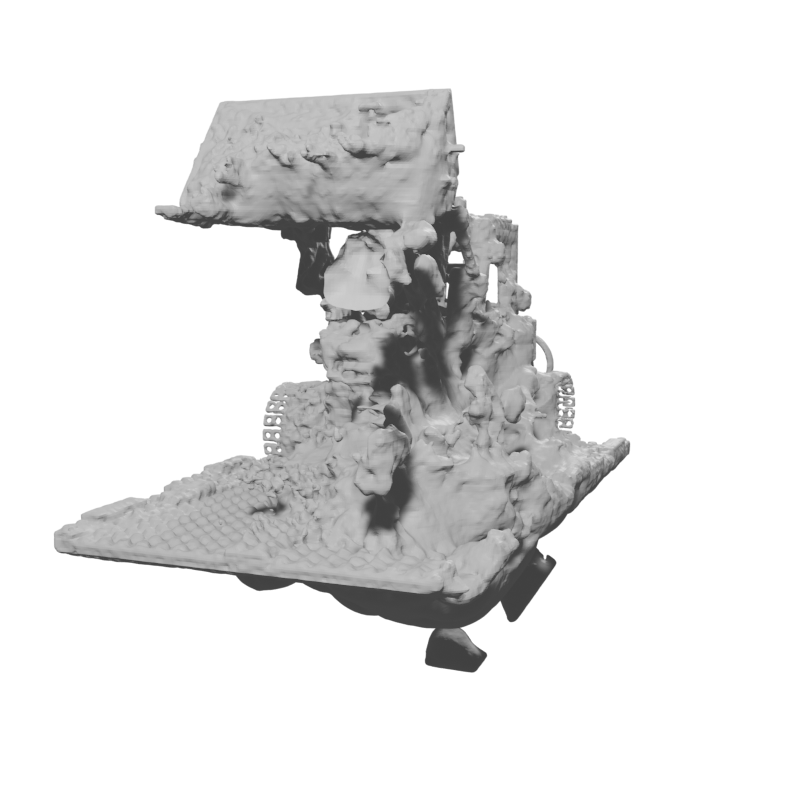}}
  \mpage{0.20}{\includegraphics[width=\linewidth]{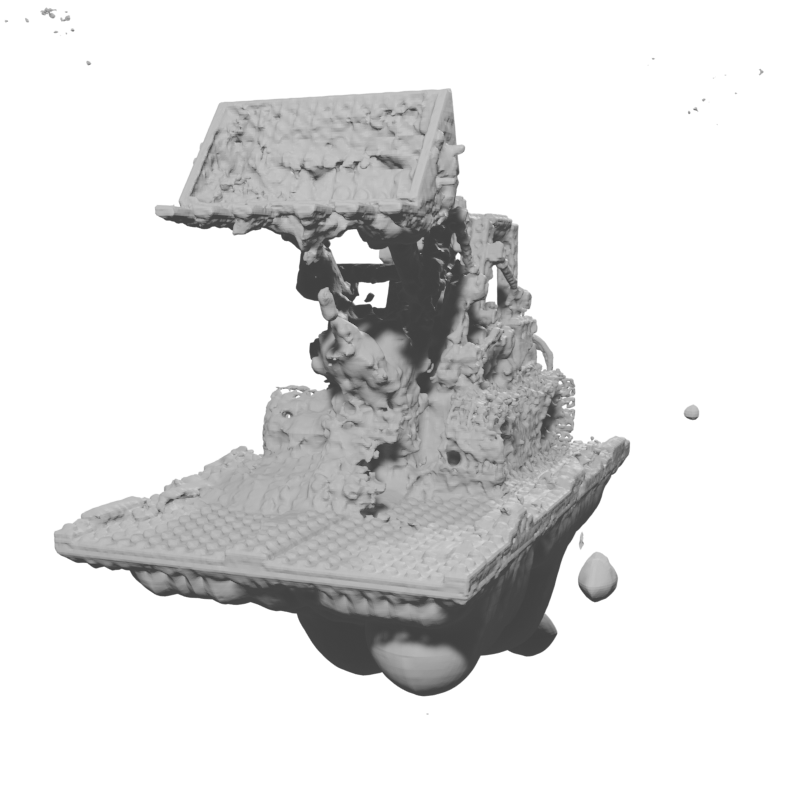}}
  \mpage{0.20}{\includegraphics[width=\linewidth]{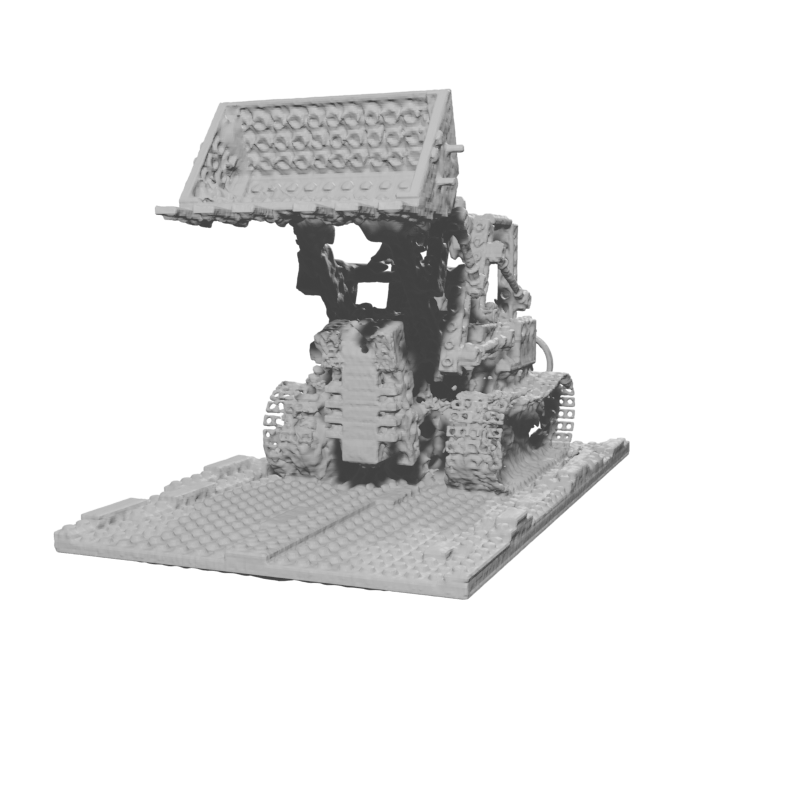}}
 \\
  
  \mpage{0.05}{\ }
  \mpage{0.195}{NeuS}
  \mpage{0.195}{MVSNeRF}
  \mpage{0.195}{SparseNeuS}
  \mpage{0.195}{Ours}
  \caption{Qualitative results of mesh reconstruction on Blender dataset~\cite{mildenhall2021nerf}. }
  \label{fig:mesh}
\end{figure}
