# Supplementary material for: HarmonicNeRF: Geometry-Informed Synthetic View Augmentation for 3D Scene Reconstruction in Driving Scenarios
Source: arXiv:2310.05483 source file (2024-07-25)
Supplement: Supplementary file 2 [file multi-view.tex]

\begin{figure}[t]
    \centering
    \rotatebox[origin=C]{90}{\parbox{20mm}{\centering \small NeuS}} 
  \mpage{0.145}{\includegraphics[width=\linewidth]{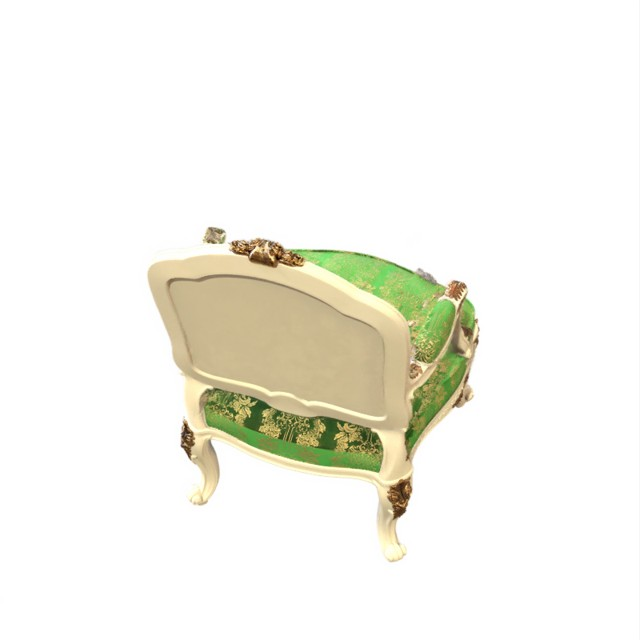}}
  \mpage{0.145}{\includegraphics[width=\linewidth]{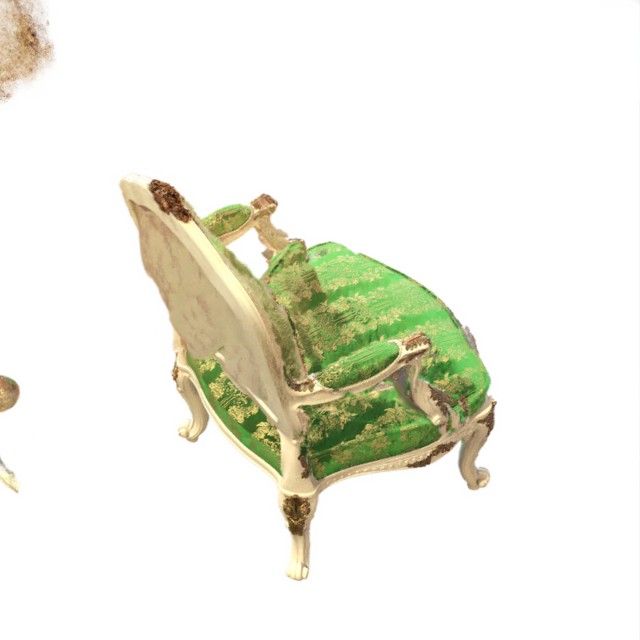}}
  \mpage{0.145}{\includegraphics[width=\linewidth]{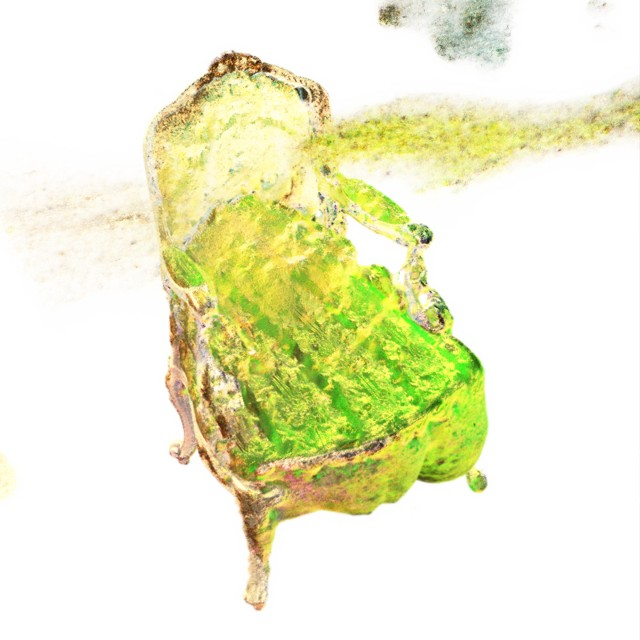}}
  \mpage{0.145}{\includegraphics[width=\linewidth]{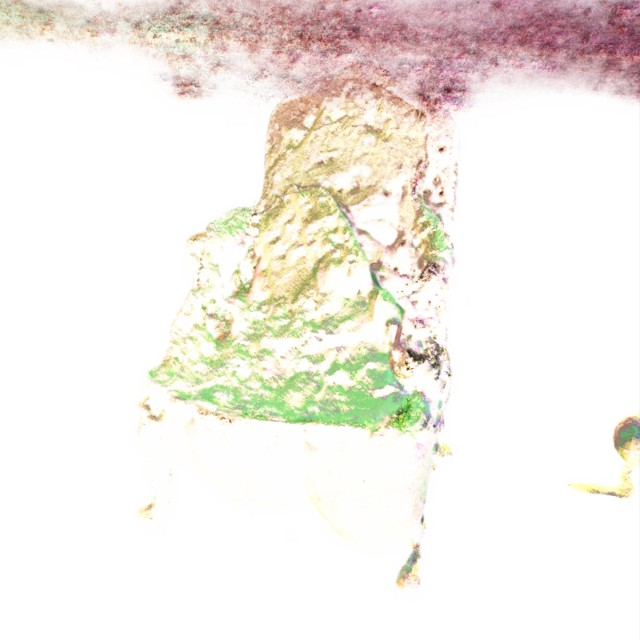}}
  \mpage{0.145}{\includegraphics[width=\linewidth]{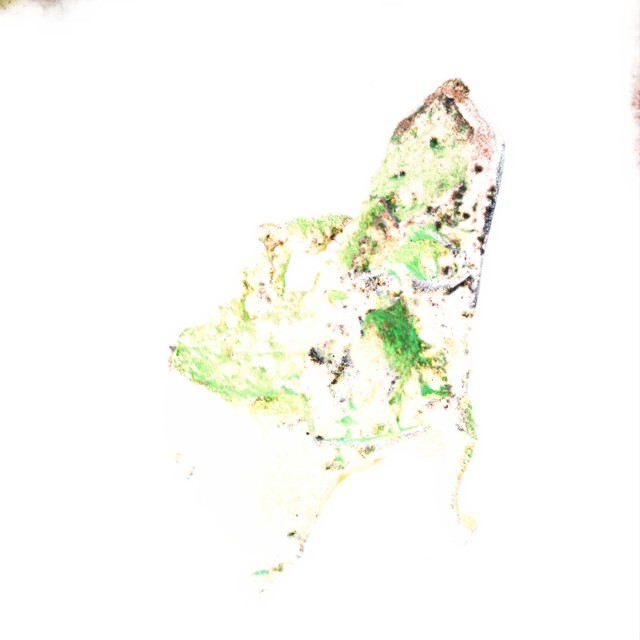}}
  \mpage{0.145}{\includegraphics[width=\linewidth]{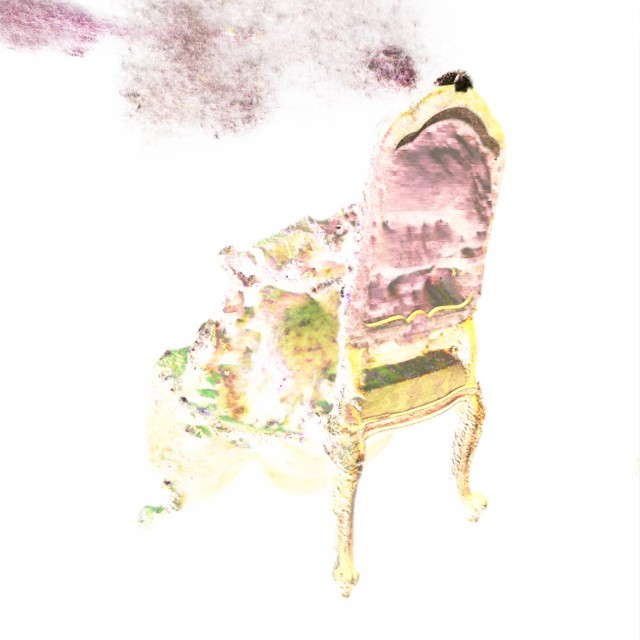}}
  \\
    \rotatebox[origin=C]{90}{\parbox{20mm}{\centering \small MVSNeRF}} 
  \mpage{0.145}{\includegraphics[width=\linewidth]{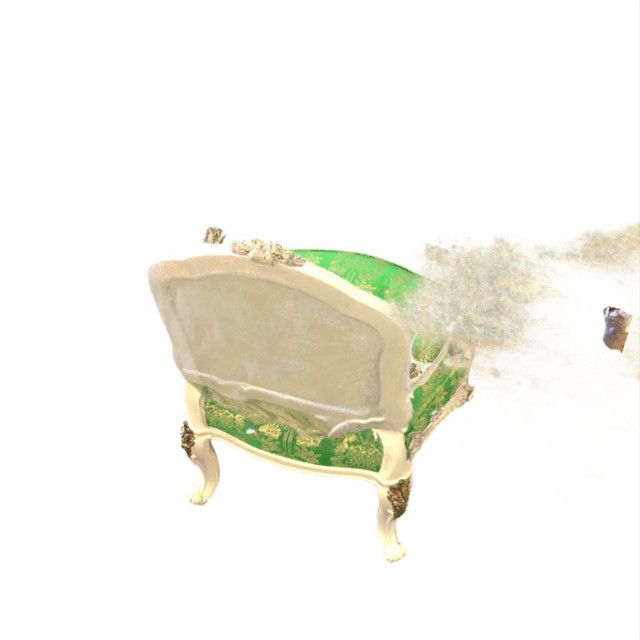}}
  \mpage{0.145}{\includegraphics[width=\linewidth]{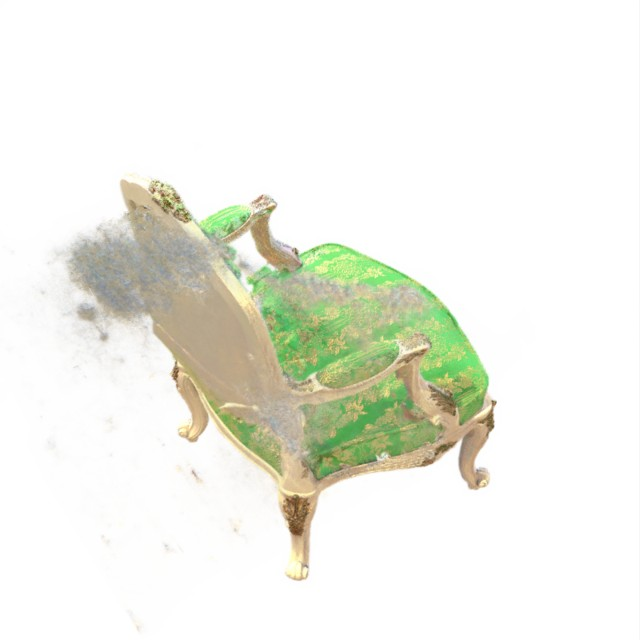}}
  \mpage{0.145}{\includegraphics[width=\linewidth]{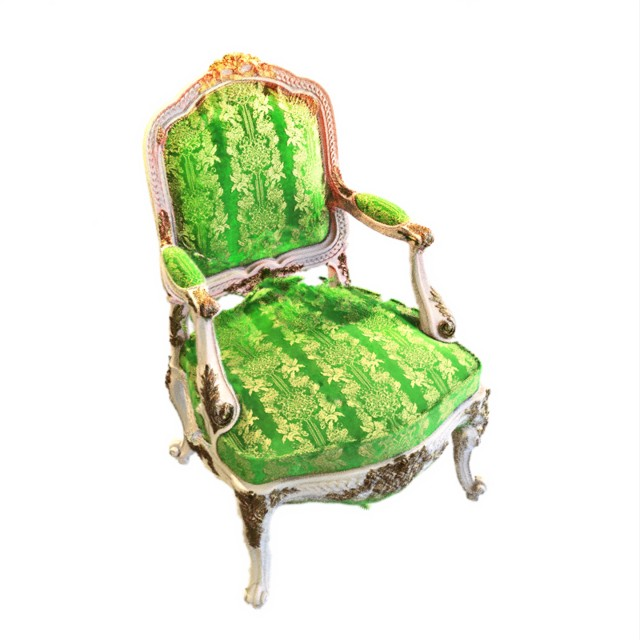}}
  \mpage{0.145}{\includegraphics[width=\linewidth]{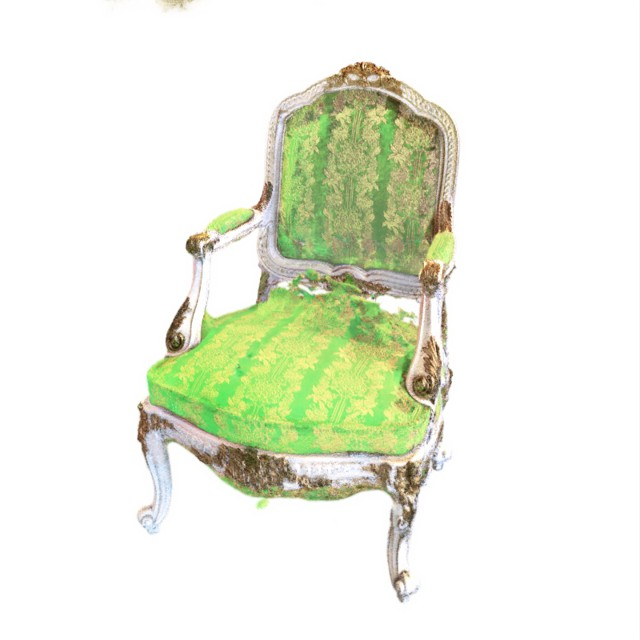}}
  \mpage{0.145}{\includegraphics[width=\linewidth]{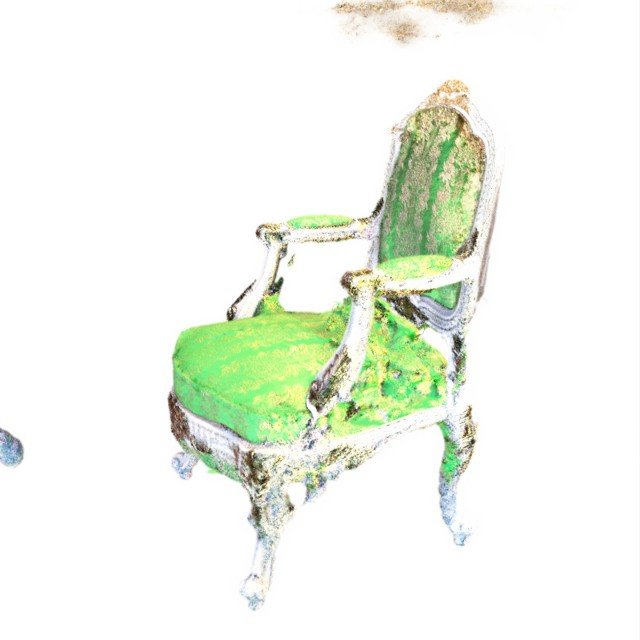}}
  \mpage{0.145}{\includegraphics[width=\linewidth]{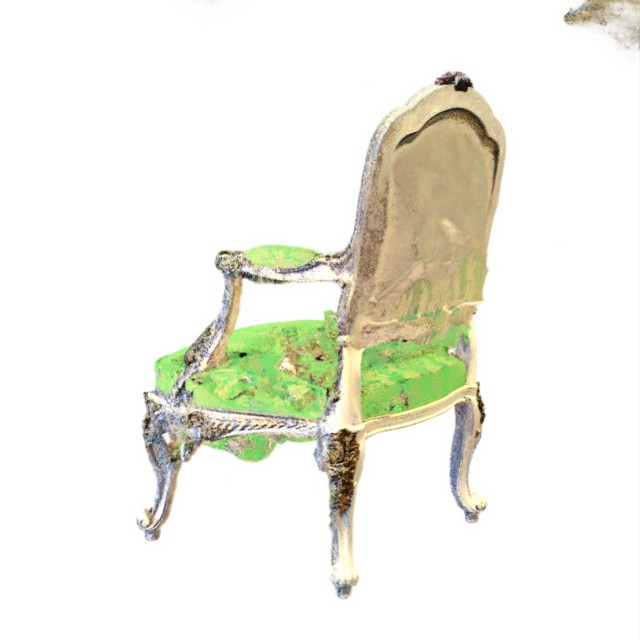}}
  \\
   \rotatebox[origin=C]{90}{\parbox{20mm}{\centering \small SparseNeuS}} 
  \mpage{0.145}{\includegraphics[width=\linewidth]{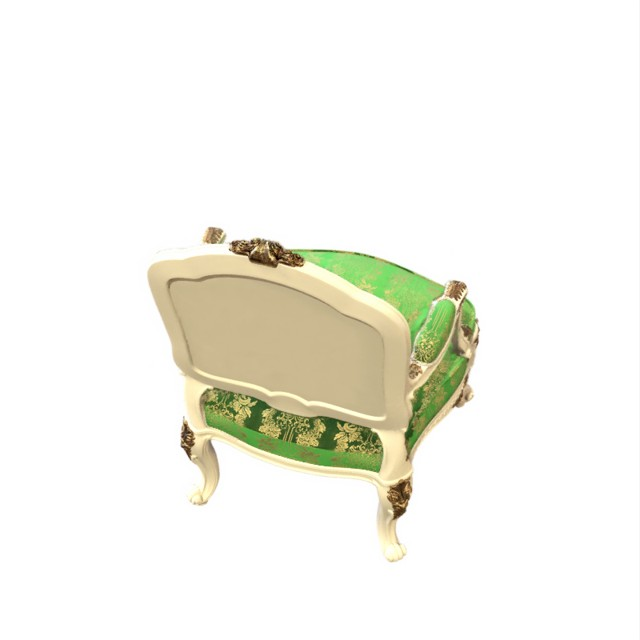}}
  \mpage{0.145}{\includegraphics[width=\linewidth]{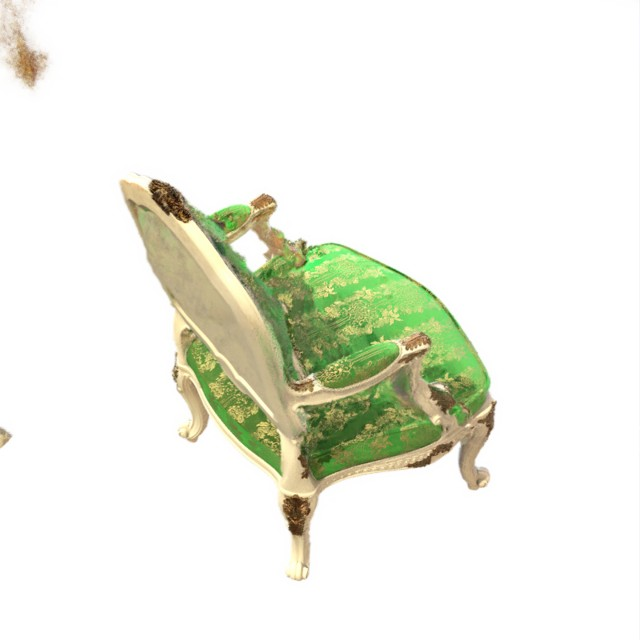}}
  \mpage{0.145}{\includegraphics[width=\linewidth]{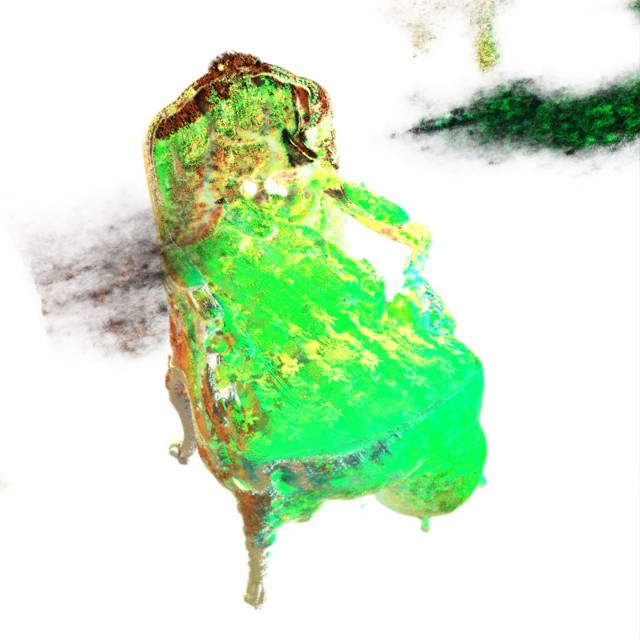}}
  \mpage{0.145}{\includegraphics[width=\linewidth]{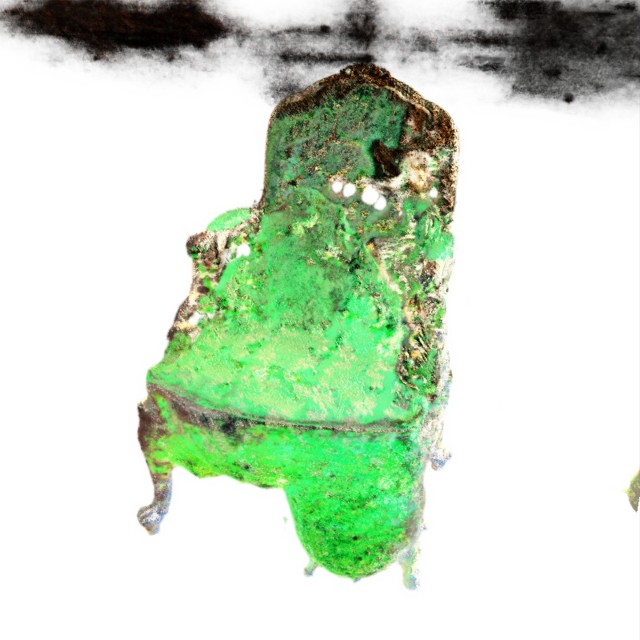}}
  \mpage{0.145}{\includegraphics[width=\linewidth]{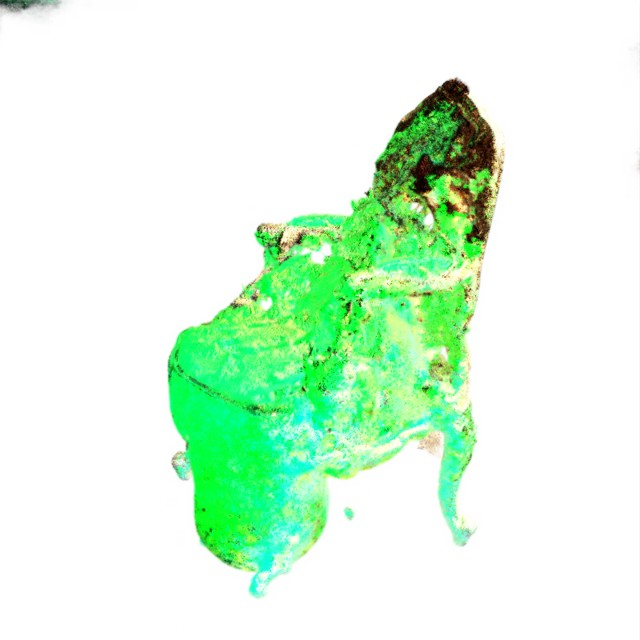}}
  \mpage{0.145}{\includegraphics[width=\linewidth]{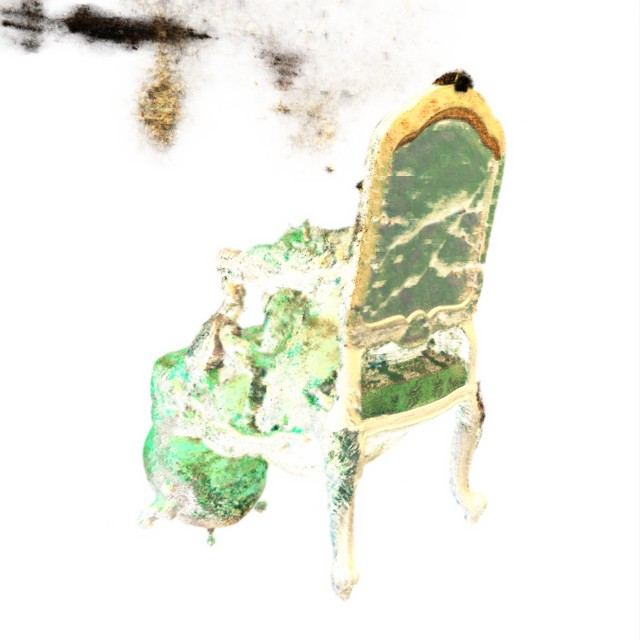}}
  \\
   \rotatebox[origin=C]{90}{\parbox{20mm}{\centering \small Ours}} 
  \mpage{0.145}{\includegraphics[width=\linewidth]{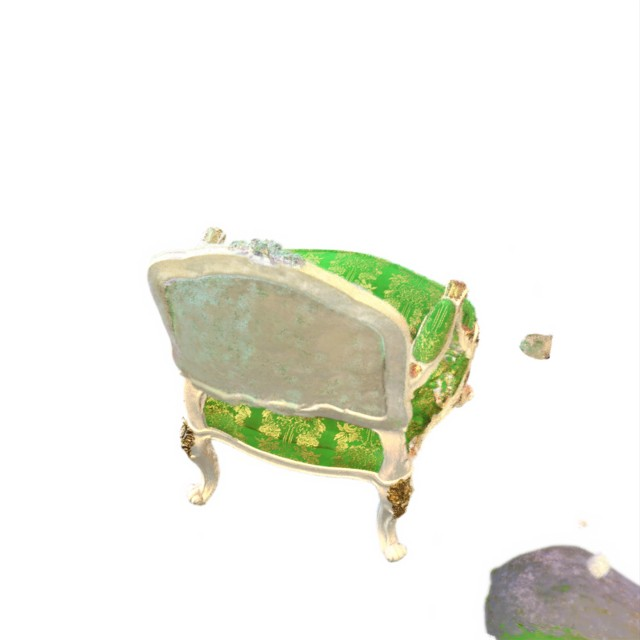}}
  \mpage{0.145}{\includegraphics[width=\linewidth]{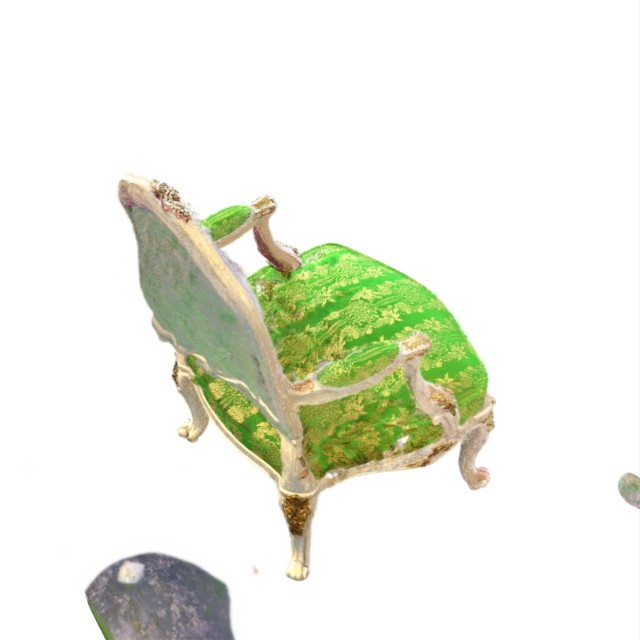}}
  \mpage{0.145}{\includegraphics[width=\linewidth]{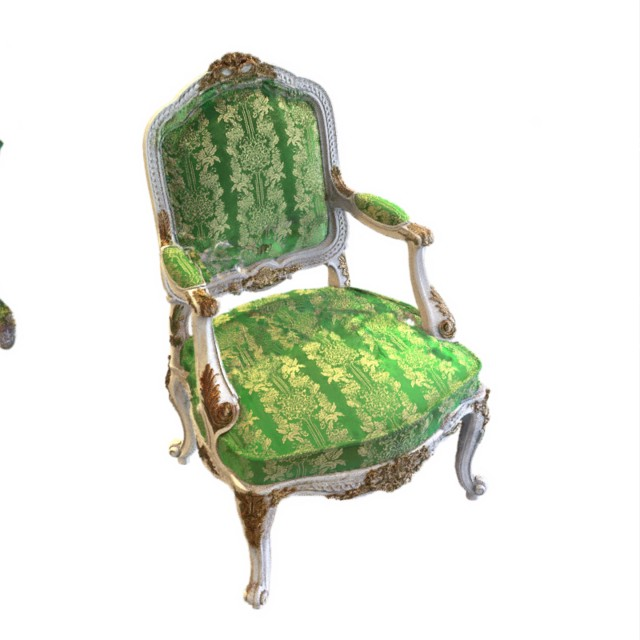}}
  \mpage{0.145}{\includegraphics[width=\linewidth]{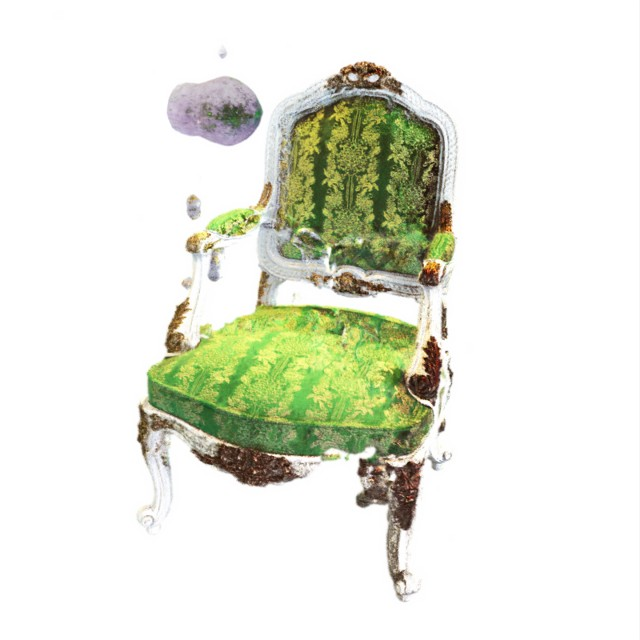}}
  \mpage{0.145}{\includegraphics[width=\linewidth]{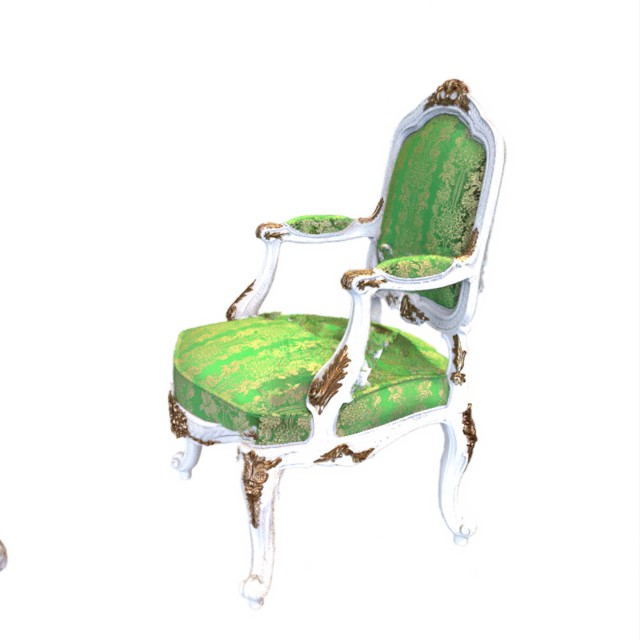}}
  \mpage{0.145}{\includegraphics[width=\linewidth]{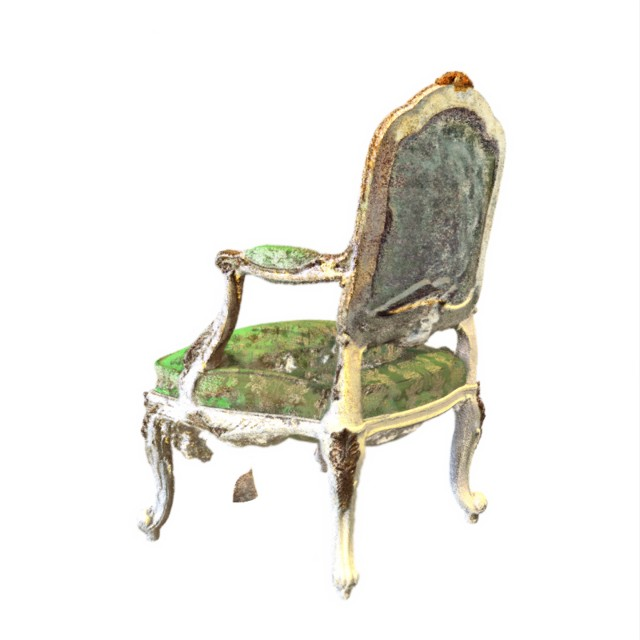}}
  \\
  \caption{Additional qualitative results of multi-view results of novel view synthesis on the Chair scene in Blender dataset~\cite{mildenhall2021nerf}. }
  \label{fig:multiview_1}
\end{figure}
