# Supplementary material for: HarmonicNeRF: Geometry-Informed Synthetic View Augmentation for 3D Scene Reconstruction in Driving Scenarios
Source: arXiv:2310.05483 source file (2024-07-25)
Supplement: Supplementary file 4 [file vis.tex]

\begin{figure}[!b]
    \centering
    \rotatebox[origin=C]{90}{\parbox{20mm}{\centering \small Ficus \\ (Blender)}} 
  \mpage{0.15}{\includegraphics[width=\linewidth]{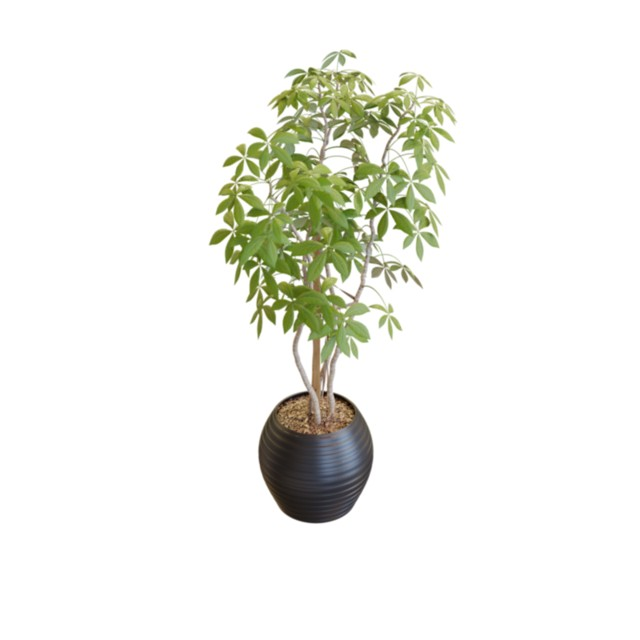}}
  \mpage{0.15}{\includegraphics[width=\linewidth]{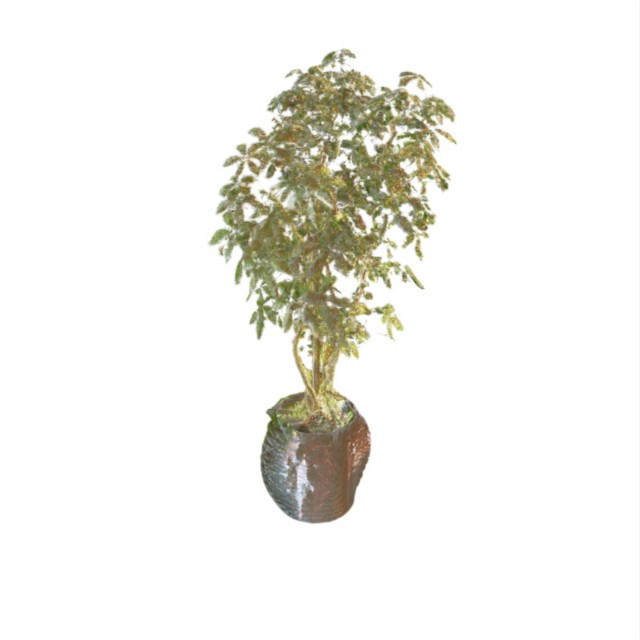}}
  \mpage{0.15}{\includegraphics[width=\linewidth]{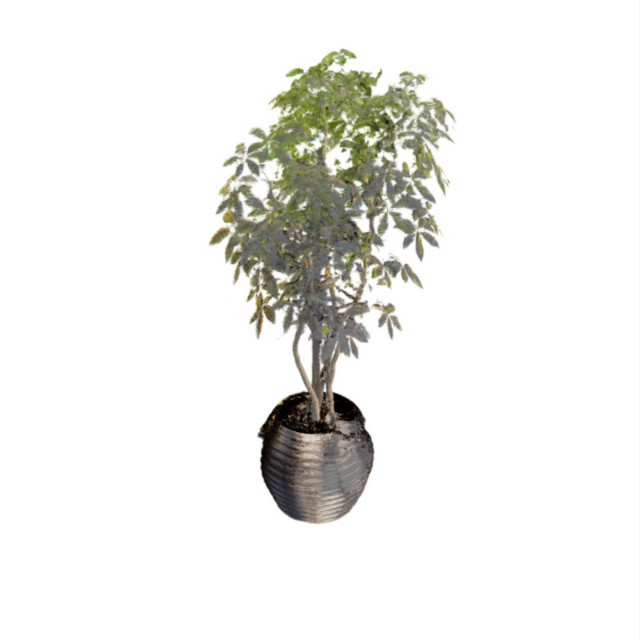}}
  \mpage{0.15}{\includegraphics[width=\linewidth]{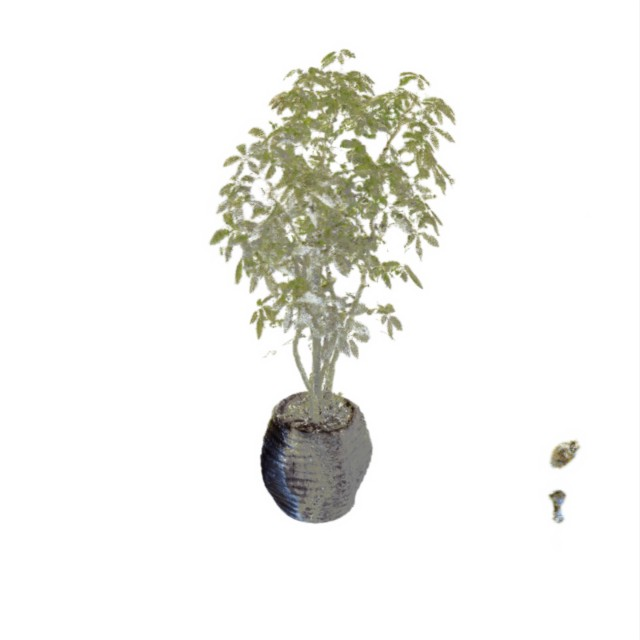}}
  \mpage{0.15}{\includegraphics[width=\linewidth]{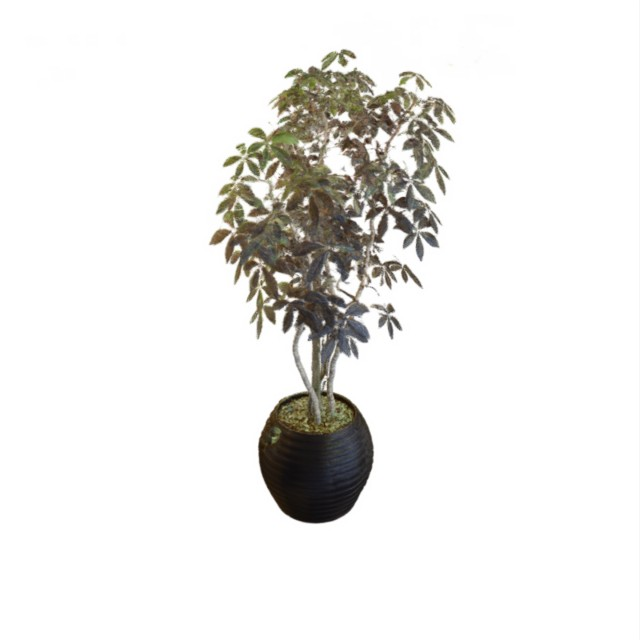}}
  \\
  \rotatebox[origin=C]{90}{\parbox{20mm}{\centering \small Hotdog \\ (Blender)}} 
  \mpage{0.15}{\includegraphics[width=\linewidth]{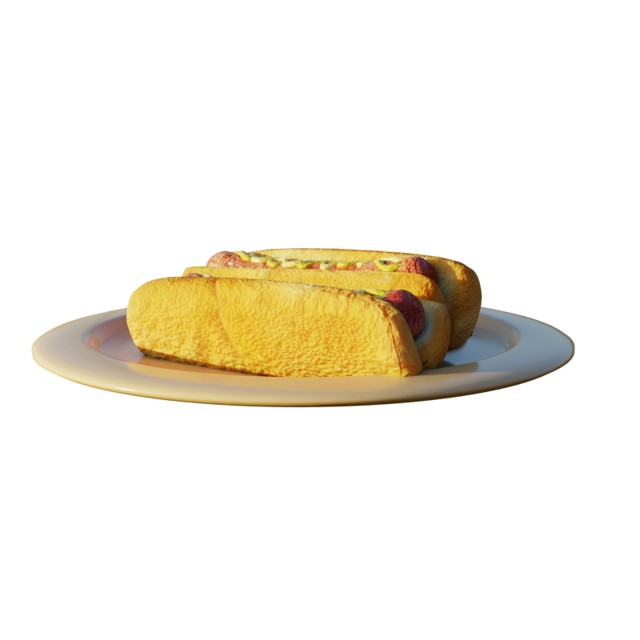}}
  \mpage{0.15}{\includegraphics[width=\linewidth]{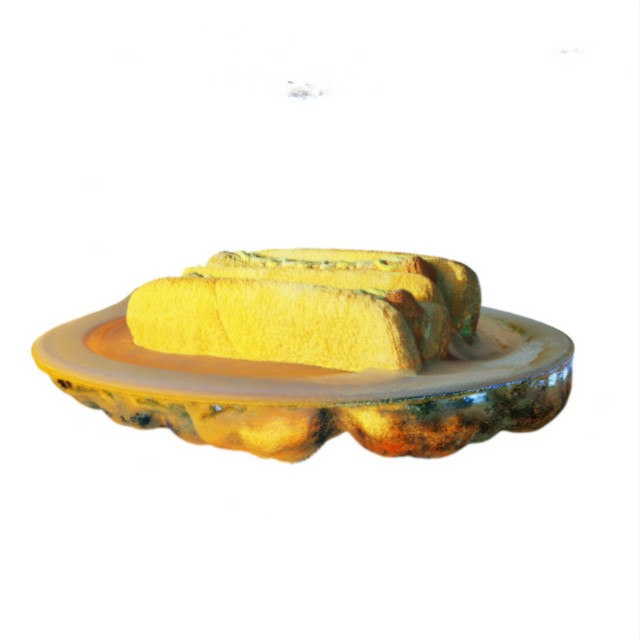}}
  \mpage{0.15}{\includegraphics[width=\linewidth]{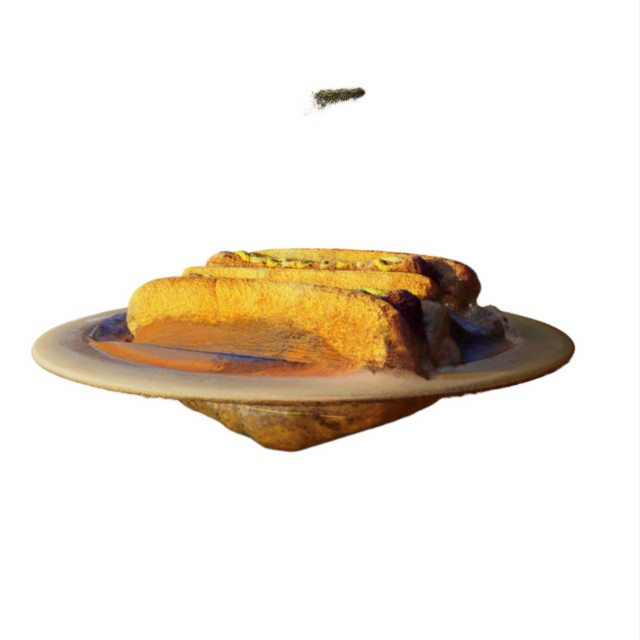}}
  \mpage{0.15}{\includegraphics[width=\linewidth]{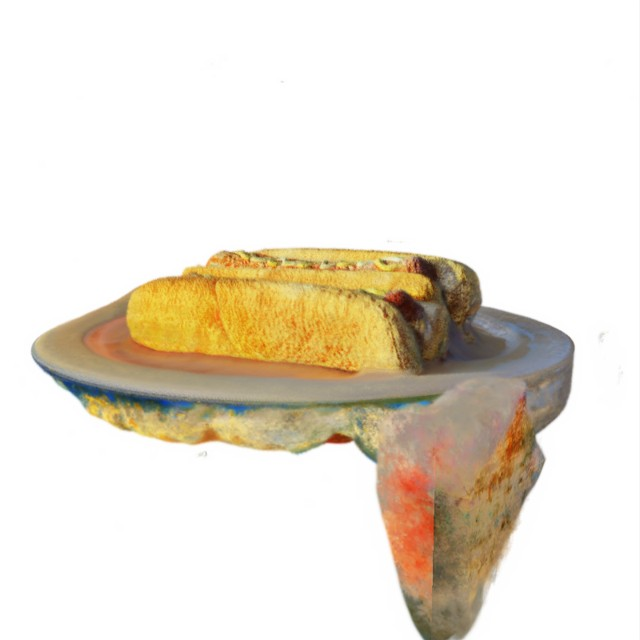}}
  \mpage{0.15}{\includegraphics[width=\linewidth]{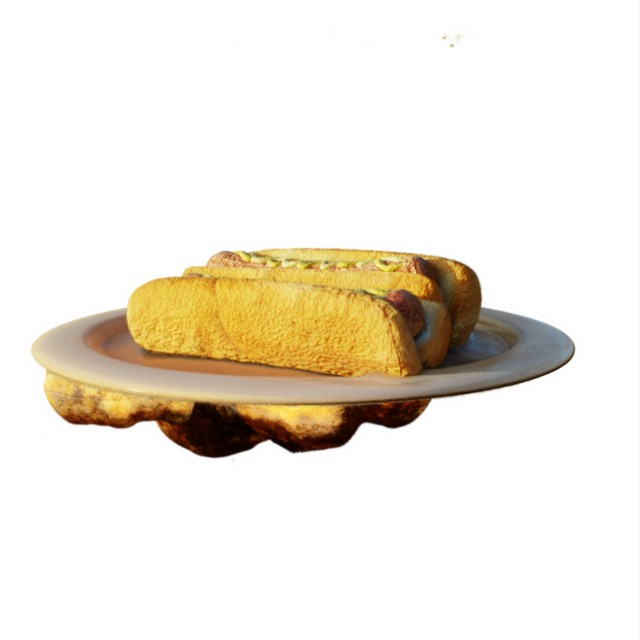}}
 \\
   \rotatebox[origin=C]{90}{\parbox{20mm}{\centering \small Lego \\ (Blender)}} 
 \mpage{0.15}{\includegraphics[width=\linewidth]{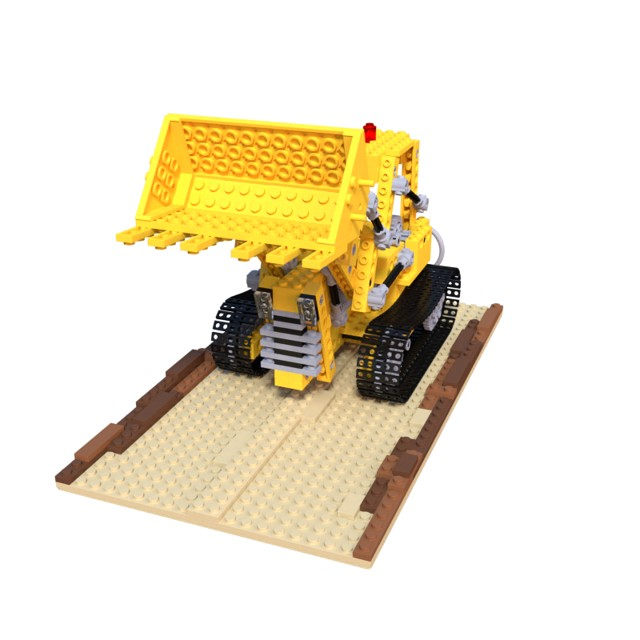}}
  \mpage{0.15}{\includegraphics[width=\linewidth]{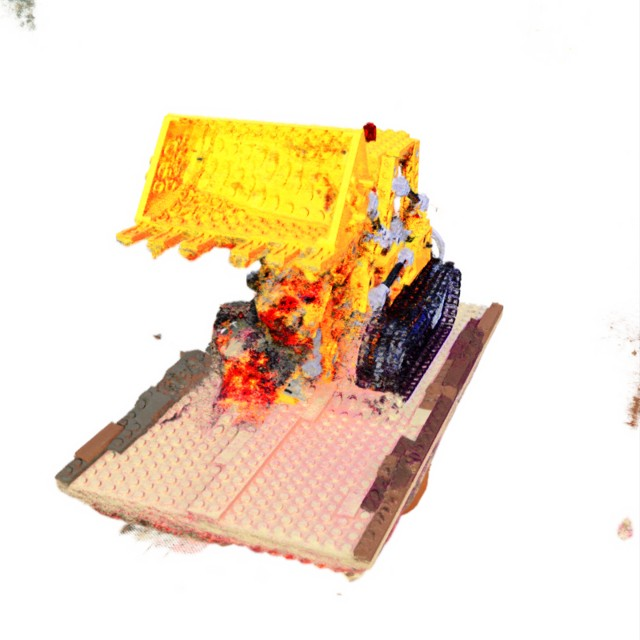}}
  \mpage{0.15}{\includegraphics[width=\linewidth]{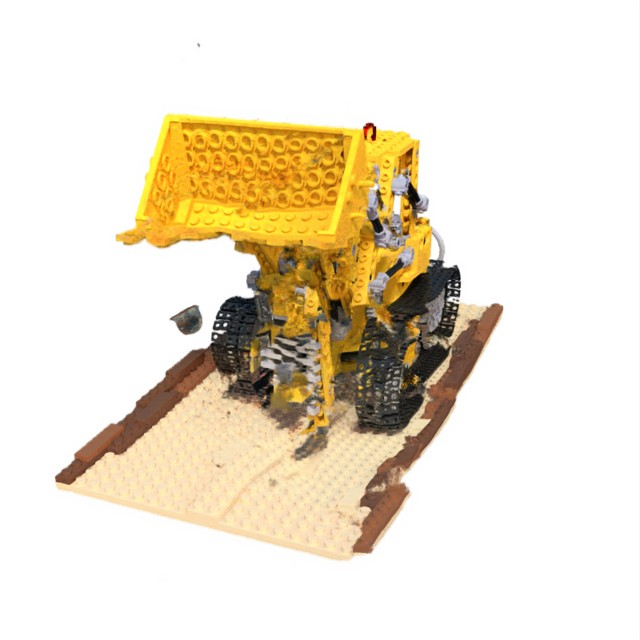}}
  \mpage{0.15}{\includegraphics[width=\linewidth]{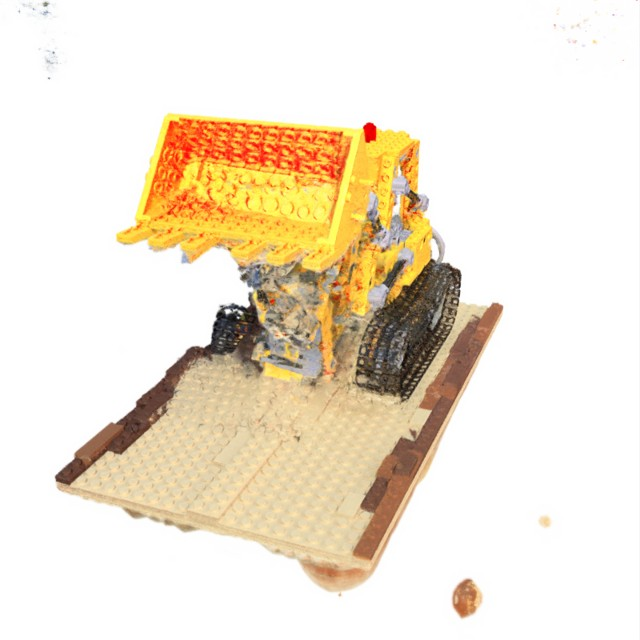}}
  \mpage{0.15}{\includegraphics[width=\linewidth]{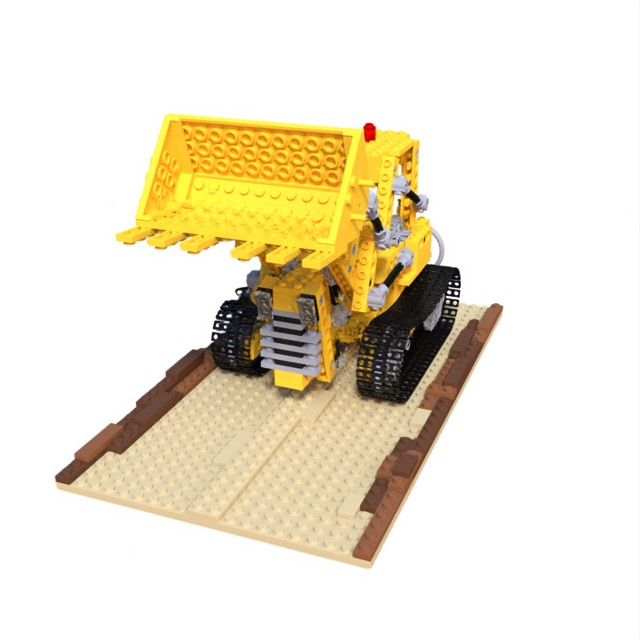}}
 \\
   \rotatebox[origin=C]{91}{\parbox{20mm}{\centering \small Materials \\ (Blender)}} 
 \mpage{0.15}{\includegraphics[width=\linewidth]{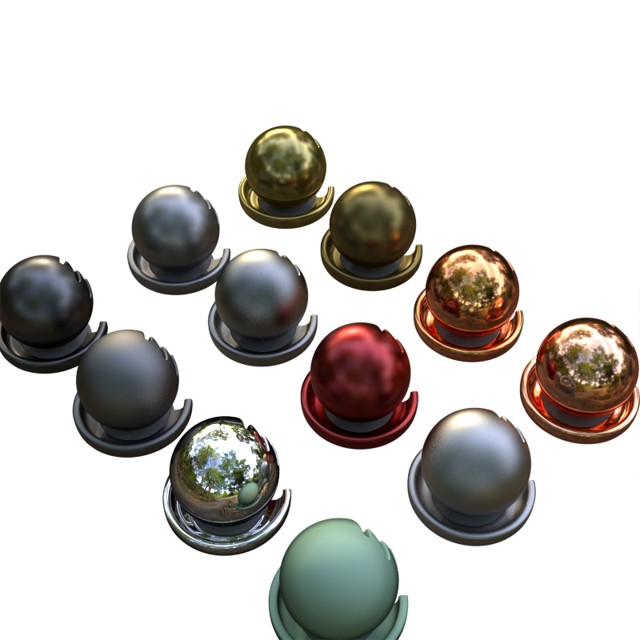}}
  \mpage{0.15}{\includegraphics[width=\linewidth]{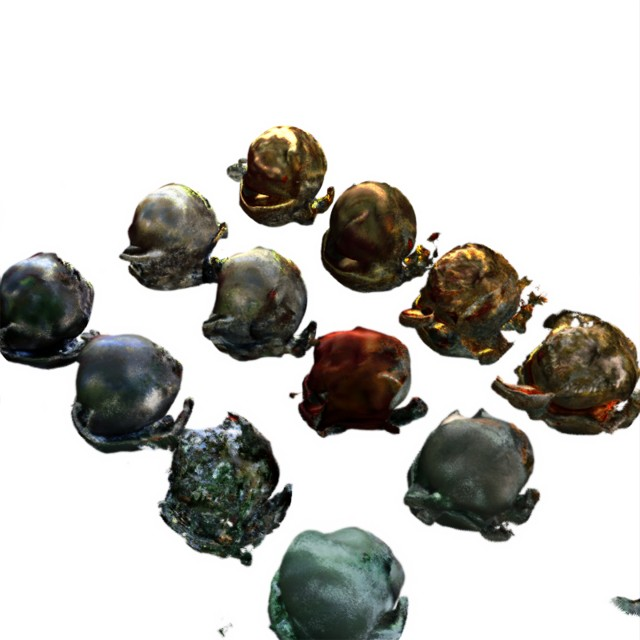}}
  \mpage{0.15}{\includegraphics[width=\linewidth]{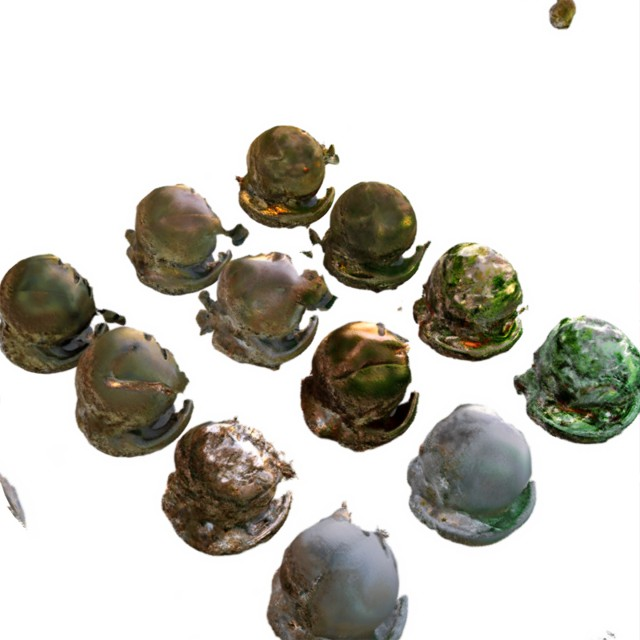}}
  \mpage{0.15}{\includegraphics[width=\linewidth]{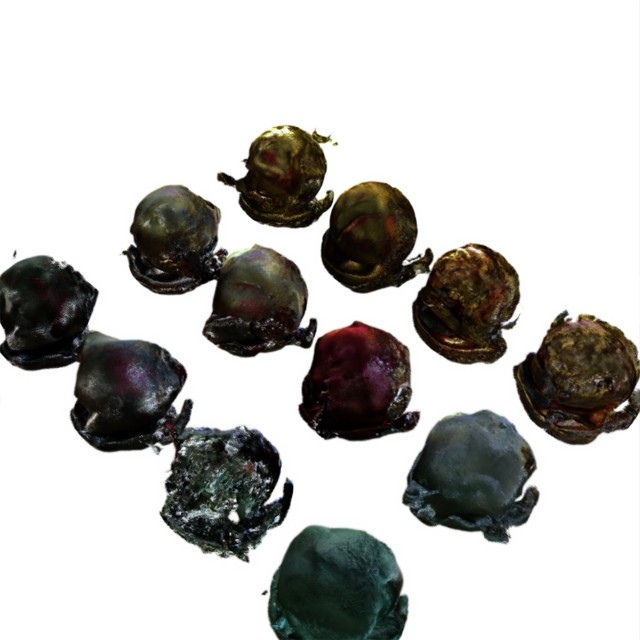}}
  \mpage{0.15}{\includegraphics[width=\linewidth]{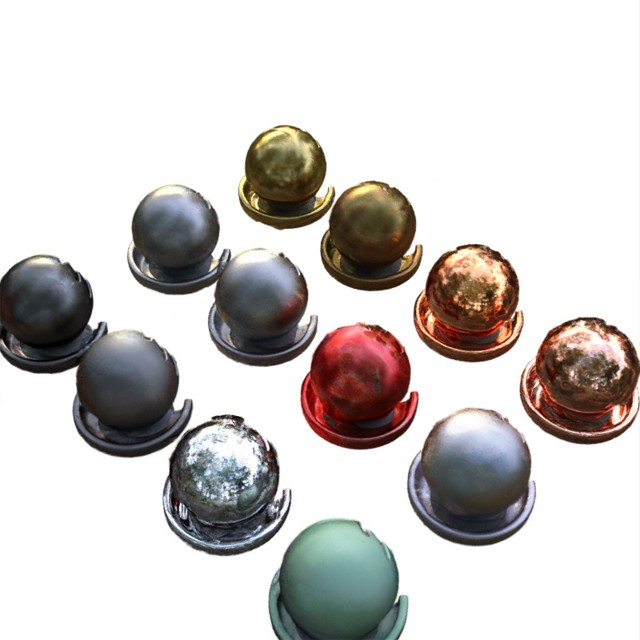}}
  \\
  
  \vspace{0.5cm}
  \mpage{0.05}{\ }
  \mpage{0.15}{Ground Truth}
  \mpage{0.15}{NeuS}
  \mpage{0.15}{MVSNeRF}
  \mpage{0.15}{SparseNeuS}
  \mpage{0.15}{Ours}
  \caption{Additional qualitative results of novel view synthesis on Blender dataset~\cite{mildenhall2021nerf}. }
  \label{fig:nvs_1}
\end{figure}
