# Supplementary material for: HarmonicNeRF: Geometry-Informed Synthetic View Augmentation for 3D Scene Reconstruction in Driving Scenarios
Source: arXiv:2310.05483 source file (2024-07-25)
Supplement: Supplementary file 5 [file supplementary.tex]

%%
%% This is file `sample-authordraft.tex',
%% generated with the docstrip utility.
%%
%% The original source files were:
%%
%% samples.dtx  (with options: `authordraft')
%% 
%% IMPORTANT NOTICE:
%% 
%% For the copyright see the source file.
%% 
%% Any modified versions of this file must be renamed
%% with new filenames distinct from sample-authordraft.tex.
%% 
%% For distribution of the original source see the terms
%% for copying and modification in the file samples.dtx.
%% 
%% This generated file may be distributed as long as the
%% original source files, as listed above, are part of the
%% same distribution. (The sources need not necessarily be
%% in the same archive or directory.)
%%
%% Commands for TeXCount
%TC:macro \cite [option:text,text]
%TC:macro \citep [option:text,text]
%TC:macro \citet [option:text,text]
%TC:envir table 0 1
%TC:envir table* 0 1
%TC:envir tabular [ignore] word
%TC:envir displaymath 0 word
%TC:envir math 0 word
%TC:envir comment 0 0
%%
%%
%% The first command in your LaTeX source must be the \documentclass command.
\documentclass[sigconf,authordraft]{acmart}
%% NOTE that a single column version may required for 
%% submission and peer review. This can be done by changing
%% the \doucmentclass[...]{acmart} in this template to 
%% \documentclass[manuscript,screen]{acmart}
%% 
%% To ensure 100% compatibility, please check the white list of
%% approved LaTeX packages to be used with the Master Article Template at
%% https://www.acm.org/publications/taps/whitelist-of-latex-packages 
%% before creating your document. The white list page provides 
%% information on how to submit additional LaTeX packages for 
%% review and adoption.
%% Fonts used in the template cannot be substituted; margin 
%% adjustments are not allowed.

%%
%% \BibTeX command to typeset BibTeX logo in the docs
\AtBeginDocument{%
  \providecommand\BibTeX{{%
    \normalfont B\kern-0.5em{\scshape i\kern-0.25em b}\kern-0.8em\TeX}}}

\settopmatter{printacmref=false} % Removes citation information below abstract
\renewcommand\footnotetextcopyrightpermission[1]{} % removes footnote with conference information in first column
\pagestyle{plain} % removes running headers 
\setcopyright{none}

\begin{document}

%%
%% The "title" command has an optional parameter,
%% allowing the author to define a "short title" to be used in page headers.
\title{Supplementary Materials: The Name of the Title is Hope}

%%
%% The "author" command and its associated commands are used to define
%% the authors and their affiliations.
%% Of note is the shared affiliation of the first two authors, and the
%% "authornote" and "authornotemark" commands
%% used to denote shared contribution to the research.
% \author{Ben Trovato}
% \authornote{Both authors contributed equally to this research.}
% \email{trovato@corporation.com}
% \orcid{1234-5678-9012}
% \author{G.K.M. Tobin}
% \authornotemark[1]
% \email{webmaster@marysville-ohio.com}
% \affiliation{%
%   \institution{Institute for Clarity in Documentation}
%   \streetaddress{P.O. Box 1212}
%   \city{Dublin}
%   \state{Ohio}
%   \country{USA}
%   \postcode{43017-6221}
% }

\author{Anonymous Authors}

\maketitle

\section{Introduction}
ACM's consolidated article template, introduced in 2017, provides a
consistent \LaTeX\ style for use across ACM publications, and
incorporates accessibility and metadata-extraction functionality
necessary for future Digital Library endeavors. Numerous ACM and
SIG-specific \LaTeX\ templates have been examined, and their unique
features incorporated into this single new template.

If you are new to publishing with ACM, this document is a valuable
guide to the process of preparing your work for publication. If you
have published with ACM before, this document provides insight and
instruction into more recent changes to the article template.

The ``\verb|acmart|'' document class can be used to prepare articles
for any ACM publication --- conference or journal, and for any stage
of publication, from review to final ``camera-ready'' copy, to the
author's own version, with {\itshape very} few changes to the source.

\section{Template Overview}
As noted in the introduction, the ``\verb|acmart|'' document class can
be used to prepare many different kinds of documentation --- a
dual-anonymous initial submission of a full-length technical paper, a
two-page SIGGRAPH Emerging Technologies abstract, a ``camera-ready''
journal article, a SIGCHI Extended Abstract, and more --- all by
selecting the appropriate {\itshape template style} and {\itshape
  template parameters}.

This document will explain the major features of the document
class. For further information, the {\itshape \LaTeX\ User's Guide} is
available from
\url{https://www.acm.org/publications/proceedings-template}.

\subsection{Template Styles}

The primary parameter given to the ``\verb|acmart|'' document class is
the {\itshape template style} which corresponds to the kind of publication
or SIG publishing the work. This parameter is enclosed in square
brackets and is a part of the {\verb|documentclass|} command:
\begin{verbatim}
  \documentclass[STYLE]{acmart}
\end{verbatim}

Journals use one of three template styles. All but three ACM journals
use the {\verb|acmsmall|} template style:
\begin{itemize}
\item {\verb|acmsmall|}: The default journal template style.
\item {\verb|acmlarge|}: Used by JOCCH and TAP.
\item {\verb|acmtog|}: Used by TOG.
\end{itemize}

The majority of conference proceedings documentation will use the {\verb|acmconf|} template style.
\begin{itemize}
\item {\verb|acmconf|}: The default proceedings template style.
\item{\verb|sigchi|}: Used for SIGCHI conference articles.
\item{\verb|sigchi-a|}: Used for SIGCHI ``Extended Abstract'' articles.
\item{\verb|sigplan|}: Used for SIGPLAN conference articles.
\end{itemize}

\subsection{Template Parameters}

In addition to specifying the {\itshape template style} to be used in
formatting your work, there are a number of {\itshape template parameters}
which modify some part of the applied template style. A complete list
of these parameters can be found in the {\itshape \LaTeX\ User's Guide.}

Frequently-used parameters, or combinations of parameters, include:
\begin{itemize}
\item {\verb|anonymous,review|}: Suitable for a ``dual-anonymous''
  conference submission. Anonymizes the work and includes line
  numbers. Use with the \verb|\acmSubmissionID| command to print the
  submission's unique ID on each page of the work.
\item{\verb|authorversion|}: Produces a version of the work suitable
  for posting by the author.
\item{\verb|screen|}: Produces colored hyperlinks.
\end{itemize}

This document uses the following string as the first command in the
source file:
\begin{verbatim}
\documentclass[sigconf,authordraft]{acmart}
\end{verbatim}

\section{Modifications}

Modifying the template --- including but not limited to: adjusting
margins, typeface sizes, line spacing, paragraph and list definitions,
and the use of the \verb|\vspace| command to manually adjust the
vertical spacing between elements of your work --- is not allowed.

{\bfseries Your document will be returned to you for revision if
  modifications are discovered.}

\section{Typefaces}

The ``\verb|acmart|'' document class requires the use of the
``Libertine'' typeface family. Your \TeX\ installation should include
this set of packages. Please do not substitute other typefaces. The
``\verb|lmodern|'' and ``\verb|ltimes|'' packages should not be used,
as they will override the built-in typeface families.

\section{Title Information}

The title of your work should use capital letters appropriately -
\url{https://capitalizemytitle.com/} has useful rules for
capitalization. Use the {\verb|title|} command to define the title of
your work. If your work has a subtitle, define it with the
{\verb|subtitle|} command.  Do not insert line breaks in your title.

If your title is lengthy, you must define a short version to be used
in the page headers, to prevent overlapping text. The \verb|title|
command has a ``short title'' parameter:
\begin{verbatim}
  \title[short title]{full title}
\end{verbatim}

\section{Authors and Affiliations}

Each author must be defined separately for accurate metadata
identification. Multiple authors may share one affiliation. Authors'
names should not be abbreviated; use full first names wherever
possible. Include authors' e-mail addresses whenever possible.

Grouping authors' names or e-mail addresses, or providing an ``e-mail
alias,'' as shown below, is not acceptable:
\begin{verbatim}
  \author{Brooke Aster, David Mehldau}
  \email{dave,judy,steve@university.edu}
  \email{firstname.lastname@phillips.org}
\end{verbatim}

The \verb|authornote| and \verb|authornotemark| commands allow a note
to apply to multiple authors --- for example, if the first two authors
of an article contributed equally to the work.

If your author list is lengthy, you must define a shortened version of
the list of authors to be used in the page headers, to prevent
overlapping text. The following command should be placed just after
the last \verb|\author{}| definition:
\begin{verbatim}
  \renewcommand{\shortauthors}{McCartney, et al.}
\end{verbatim}
Omitting this command will force the use of a concatenated list of all
of the authors' names, which may result in overlapping text in the
page headers.

The article template's documentation, available at
\url{https://www.acm.org/publications/proceedings-template}, has a
complete explanation of these commands and tips for their effective
use.

Note that authors' addresses are mandatory for journal articles.

\section{Rights Information}

Authors of any work published by ACM will need to complete a rights
form. Depending on the kind of work, and the rights management choice
made by the author, this may be copyright transfer, permission,
license, or an OA (open access) agreement.

Regardless of the rights management choice, the author will receive a
copy of the completed rights form once it has been submitted. This
form contains \LaTeX\ commands that must be copied into the source
document. When the document source is compiled, these commands and
their parameters add formatted text to several areas of the final
document:
\begin{itemize}
\item the ``ACM Reference Format'' text on the first page.
\item the ``rights management'' text on the first page.
\item the conference information in the page header(s).
\end{itemize}

Rights information is unique to the work; if you are preparing several
works for an event, make sure to use the correct set of commands with
each of the works.

The ACM Reference Format text is required for all articles over one
page in length, and is optional for one-page articles (abstracts).

\section{CCS Concepts and User-Defined Keywords}

Two elements of the ``acmart'' document class provide powerful
taxonomic tools for you to help readers find your work in an online
search.

The ACM Computing Classification System ---
\url{https://www.acm.org/publications/class-2012} --- is a set of
classifiers and concepts that describe the computing
discipline. Authors can select entries from this classification
system, via \url{https://dl.acm.org/ccs/ccs.cfm}, and generate the
commands to be included in the \LaTeX\ source.

User-defined keywords are a comma-separated list of words and phrases
of the authors' choosing, providing a more flexible way of describing
the research being presented.

CCS concepts and user-defined keywords are required for for all
articles over two pages in length, and are optional for one- and
two-page articles (or abstracts).

\section{Sectioning Commands}

Your work should use standard \LaTeX\ sectioning commands:
\verb|section|, \verb|subsection|, \verb|subsubsection|, and
\verb|paragraph|. They should be numbered; do not remove the numbering
from the commands.

Simulating a sectioning command by setting the first word or words of
a paragraph in boldface or italicized text is {\bfseries not allowed.}

\section{Tables}

The ``\verb|acmart|'' document class includes the ``\verb|booktabs|''
package --- \url{https://ctan.org/pkg/booktabs} --- for preparing
high-quality tables.

Table captions are placed {\itshape above} the table.

Because tables cannot be split across pages, the best placement for
them is typically the top of the page nearest their initial cite.  To
ensure this proper ``floating'' placement of tables, use the
environment \textbf{table} to enclose the table's contents and the
table caption.  The contents of the table itself must go in the
\textbf{tabular} environment, to be aligned properly in rows and
columns, with the desired horizontal and vertical rules.  Again,
detailed instructions on \textbf{tabular} material are found in the
\textit{\LaTeX\ User's Guide}.

Immediately following this sentence is the point at which
Table~\ref{tab:freq} is included in the input file; compare the
placement of the table here with the table in the printed output of
this document.

\begin{table}
  \caption{Frequency of Special Characters}
  \label{tab:freq}
  \begin{tabular}{ccl}
    \toprule
    Non-English or Math&Frequency&Comments\\
    \midrule
    \O & 1 in 1,000& For Swedish names\\
    $\pi$ & 1 in 5& Common in math\\
    \$ & 4 in 5 & Used in business\\
    $\Psi^2_1$ & 1 in 40,000& Unexplained usage\\
  \bottomrule
\end{tabular}
\end{table}

To set a wider table, which takes up the whole width of the page's
live area, use the environment \textbf{table*} to enclose the table's
contents and the table caption.  As with a single-column table, this
wide table will ``float'' to a location deemed more
desirable. Immediately following this sentence is the point at which
Table~\ref{tab:commands} is included in the input file; again, it is
instructive to compare the placement of the table here with the table
in the printed output of this document.

\begin{table*}
  \caption{Some Typical Commands}
  \label{tab:commands}
  \begin{tabular}{ccl}
    \toprule
    Command &A Number & Comments\\
    \midrule
    \texttt{{\char'134}author} & 100& Author \\
    \texttt{{\char'134}table}& 300 & For tables\\
    \texttt{{\char'134}table*}& 400& For wider tables\\
    \bottomrule
  \end{tabular}
\end{table*}

Always use midrule to separate table header rows from data rows, and
use it only for this purpose. This enables assistive technologies to
recognise table headers and support their users in navigating tables
more easily.

\section{Math Equations}
You may want to display math equations in three distinct styles:
inline, numbered or non-numbered display.  Each of the three are
discussed in the next sections.

\subsection{Inline (In-text) Equations}
A formula that appears in the running text is called an inline or
in-text formula.  It is produced by the \textbf{math} environment,
which can be invoked with the usual
\texttt{{\char'134}begin\,\ldots{\char'134}end} construction or with
the short form \texttt{\$\,\ldots\$}. You can use any of the symbols
and structures, from $\alpha$ to $\omega$, available in
\LaTeX~\cite{Lamport:LaTeX}; this section will simply show a few
examples of in-text equations in context. Notice how this equation:
\begin{math}
  \lim_{n\rightarrow \infty}x=0
\end{math},
set here in in-line math style, looks slightly different when
set in display style.  (See next section).

\subsection{Display Equations}
A numbered display equation---one set off by vertical space from the
text and centered horizontally---is produced by the \textbf{equation}
environment. An unnumbered display equation is produced by the
\textbf{displaymath} environment.

Again, in either environment, you can use any of the symbols and
structures available in \LaTeX\@; this section will just give a couple
of examples of display equations in context.  First, consider the
equation, shown as an inline equation above:
\begin{equation}
  \lim_{n\rightarrow \infty}x=0
\end{equation}
Notice how it is formatted somewhat differently in
the \textbf{displaymath}
environment.  Now, we'll enter an unnumbered equation:
\begin{displaymath}
  \sum_{i=0}^{\infty} x + 1
\end{displaymath}
and follow it with another numbered equation:
\begin{equation}
  \sum_{i=0}^{\infty}x_i=\int_{0}^{\pi+2} f
\end{equation}
just to demonstrate \LaTeX's able handling of numbering.

\section{Figures}

The ``\verb|figure|'' environment should be used for figures. One or
more images can be placed within a figure. If your figure contains
third-party material, you must clearly identify it as such, as shown
in the example below.

\begin{figure}[h]
  \centering
    \fbox{\rule{0pt}{2.5in} \rule{0.9\linewidth}{0pt}}
  \caption{Example of caption}
\end{figure}

Your figures should contain a caption which describes the figure to
the reader.

Figure captions are placed {\itshape below} the figure.

Every figure should also have a figure description unless it is purely
decorative. These descriptions convey what’s in the image to someone
who cannot see it. They are also used by search engine crawlers for
indexing images, and when images cannot be loaded.

A figure description must be unformatted plain text less than 2000
characters long (including spaces).  {\bfseries Figure descriptions
  should not repeat the figure caption – their purpose is to capture
  important information that is not already provided in the caption or
  the main text of the paper.} For figures that convey important and
complex new information, a short text description may not be
adequate. More complex alternative descriptions can be placed in an
appendix and referenced in a short figure description. For example,
provide a data table capturing the information in a bar chart, or a
structured list representing a graph.  For additional information
regarding how best to write figure descriptions and why doing this is
so important, please see
\url{https://www.acm.org/publications/taps/describing-figures/}.

\subsection{The ``Teaser Figure''}

A ``teaser figure'' is an image, or set of images in one figure, that
are placed after all author and affiliation information, and before
the body of the article, spanning the page. If you wish to have such a
figure in your article, place the command immediately before the
\verb|\maketitle| command:
\begin{verbatim}
  \begin{teaserfigure}
    \includegraphics[width=\textwidth]{sampleteaser}
    \caption{figure caption}
    \Description{figure description}
  \end{teaserfigure}
\end{verbatim}

\section{Citations and Bibliographies}

The use of \BibTeX\ for the preparation and formatting of one's
references is strongly recommended. Authors' names should be complete
--- use full first names (``Donald E. Knuth'') not initials
(``D. E. Knuth'') --- and the salient identifying features of a
reference should be included: title, year, volume, number, pages,
article DOI, etc.

The bibliography is included in your source document with these two
commands, placed just before the \verb|\end{document}| command:
\begin{verbatim}
  \bibliographystyle{ACM-Reference-Format}
  \bibliography{bibfile}
\end{verbatim}
where ``\verb|bibfile|'' is the name, without the ``\verb|.bib|''
suffix, of the \BibTeX\ file.

Citations and references are numbered by default. A small number of
ACM publications have citations and references formatted in the
``author year'' style; for these exceptions, please include this
command in the {\bfseries preamble} (before the command
``\verb|\begin{document}|'') of your \LaTeX\ source:
\begin{verbatim}
  \citestyle{acmauthoryear}
\end{verbatim}

  Some examples.  A paginated journal article \cite{Abril07}, an
  enumerated journal article \cite{Cohen07}, a reference to an entire
  issue \cite{JCohen96}, a monograph (whole book) \cite{Kosiur01}, a
  monograph/whole book in a series (see 2a in spec. document)
  \cite{Harel79}, a divisible-book such as an anthology or compilation
  \cite{Editor00} followed by the same example, however we only output
  the series if the volume number is given \cite{Editor00a} (so
  Editor00a's series should NOT be present since it has no vol. no.),
  a chapter in a divisible book \cite{Spector90}, a chapter in a
  divisible book in a series \cite{Douglass98}, a multi-volume work as
  book \cite{Knuth97}, a couple of articles in a proceedings (of a
  conference, symposium, workshop for example) (paginated proceedings
  article) \cite{Andler79, Hagerup1993}, a proceedings article with
  all possible elements \cite{Smith10}, an example of an enumerated
  proceedings article \cite{VanGundy07}, an informally published work
  \cite{Harel78}, a couple of preprints \cite{Bornmann2019,
    AnzarootPBM14}, a doctoral dissertation \cite{Clarkson85}, a
  master's thesis: \cite{anisi03}, an online document / world wide web
  resource \cite{Thornburg01, Ablamowicz07, Poker06}, a video game
  (Case 1) \cite{Obama08} and (Case 2) \cite{Novak03} and \cite{Lee05}
  and (Case 3) a patent \cite{JoeScientist001}, work accepted for
  publication \cite{rous08}, 'YYYYb'-test for prolific author
  \cite{SaeediMEJ10} and \cite{SaeediJETC10}. Other cites might
  contain 'duplicate' DOI and URLs (some SIAM articles)
  \cite{Kirschmer:2010:AEI:1958016.1958018}. Boris / Barbara Beeton:
  multi-volume works as books \cite{MR781536} and \cite{MR781537}. A
  couple of citations with DOIs:
  \cite{2004:ITE:1009386.1010128,Kirschmer:2010:AEI:1958016.1958018}. Online
  citations: \cite{TUGInstmem, Thornburg01, CTANacmart}. Artifacts:
  \cite{R} and \cite{UMassCitations}.

\section{Acknowledgments}

Identification of funding sources and other support, and thanks to
individuals and groups that assisted in the research and the
preparation of the work should be included in an acknowledgment
section, which is placed just before the reference section in your
document.

This section has a special environment:
\begin{verbatim}
  \begin{acks}
  ...
  \end{acks}
\end{verbatim}
so that the information contained therein can be more easily collected
during the article metadata extraction phase, and to ensure
consistency in the spelling of the section heading.

Authors should not prepare this section as a numbered or unnumbered {\verb|\section|}; please use the ``{\verb|acks|}'' environment.

\section{Appendices}

If your work needs an appendix, add it before the
``\verb|\end{document}|'' command at the conclusion of your source
document.

Start the appendix with the ``\verb|appendix|'' command:
\begin{verbatim}
  \appendix
\end{verbatim}
and note that in the appendix, sections are lettered, not
numbered. This document has two appendices, demonstrating the section
and subsection identification method.

\section{Multi-language papers}

Papers may be written in languages other than English or include
titles, subtitles, keywords and abstracts in different languages (as a
rule, a paper in a language other than English should include an
English title and an English abstract).  Use \verb|language=...| for
every language used in the paper.  The last language indicated is the
main language of the paper.  For example, a French paper with
additional titles and abstracts in English and German may start with
the following command
\begin{verbatim}
\documentclass[sigconf, language=english, language=german,
               language=french]{acmart}
\end{verbatim}

The title, subtitle, keywords and abstract will be typeset in the main
language of the paper.  The commands \verb|\translatedXXX|, \verb|XXX|
begin title, subtitle and keywords, can be used to set these elements
in the other languages.  The environment \verb|translatedabstract| is
used to set the translation of the abstract.  These commands and
environment have a mandatory first argument: the language of the
second argument.  See \verb|sample-sigconf-i13n.tex| file for examples
of their usage.

\section{SIGCHI Extended Abstracts}

The ``\verb|sigchi-a|'' template style (available only in \LaTeX\ and
not in Word) produces a landscape-orientation formatted article, with
a wide left margin. Three environments are available for use with the
``\verb|sigchi-a|'' template style, and produce formatted output in
the margin:
\begin{itemize}
\item {\verb|sidebar|}:  Place formatted text in the margin.
\item {\verb|marginfigure|}: Place a figure in the margin.
\item {\verb|margintable|}: Place a table in the margin.
\end{itemize}

%%
%% The acknowledgments section is defined using the "acks" environment
%% (and NOT an unnumbered section). This ensures the proper
%% identification of the section in the article metadata, and the
%% consistent spelling of the heading.
% \begin{acks}
% To Robert, for the bagels and explaining CMYK and color spaces.
% \end{acks}

%%
%% The next two lines define the bibliography style to be used, and
%% the bibliography file.
\bibliographystyle{ACM-Reference-Format}
\bibliography{sample-base}

%%
%% If your work has an appendix, this is the place to put it.
% \appendix

% \section{Research Methods}

% \subsection{Part One}

% Lorem ipsum dolor sit amet, consectetur adipiscing elit. Morbi
% malesuada, quam in pulvinar varius, metus nunc fermentum urna, id
% sollicitudin purus odio sit amet enim. Aliquam ullamcorper eu ipsum
% vel mollis. Curabitur quis dictum nisl. Phasellus vel semper risus, et
% lacinia dolor. Integer ultricies commodo sem nec semper.

% \subsection{Part Two}

% Etiam commodo feugiat nisl pulvinar pellentesque. Etiam auctor sodales
% ligula, non varius nibh pulvinar semper. Suspendisse nec lectus non
% ipsum convallis congue hendrerit vitae sapien. Donec at laoreet
% eros. Vivamus non purus placerat, scelerisque diam eu, cursus
% ante. Etiam aliquam tortor auctor efficitur mattis.

% \section{Online Resources}

% Nam id fermentum dui. Suspendisse sagittis tortor a nulla mollis, in
% pulvinar ex pretium. Sed interdum orci quis metus euismod, et sagittis
% enim maximus. Vestibulum gravida massa ut felis suscipit
% congue. Quisque mattis elit a risus ultrices commodo venenatis eget
% dui. Etiam sagittis eleifend elementum.

% Nam interdum magna at lectus dignissim, ac dignissim lorem
% rhoncus. Maecenas eu arcu ac neque placerat aliquam. Nunc pulvinar
% massa et mattis lacinia.

\end{document}
