# Supplementary material for: HarmonicNeRF: Geometry-Informed Synthetic View Augmentation for 3D Scene Reconstruction in Driving Scenarios
Source: arXiv:2310.05483 source file (2024-07-25)
Supplement: Supplementary file 6 [file NumberOfImages_vis.tex]

\begin{figure}[!b]
    \centering
    \rotatebox[origin=C]{90}{\parbox{20mm}{\centering \small Chair}} 
  \mpage{0.12}{\includegraphics[width=\linewidth]{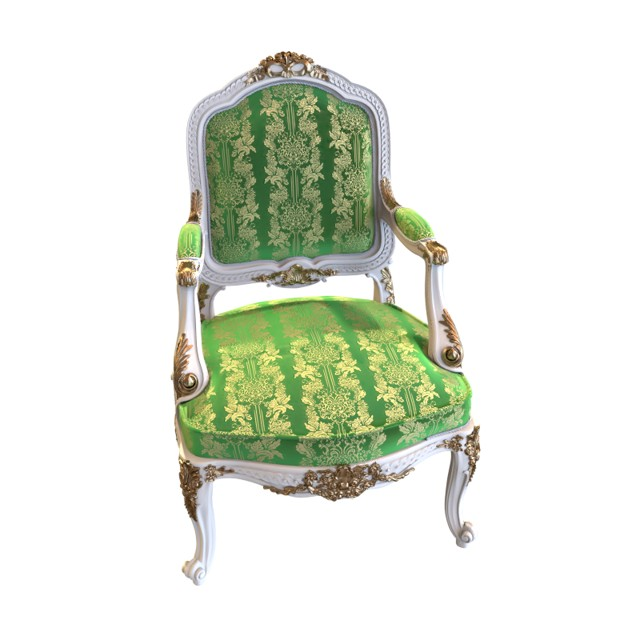}}
  \mpage{0.12}{\includegraphics[width=\linewidth]{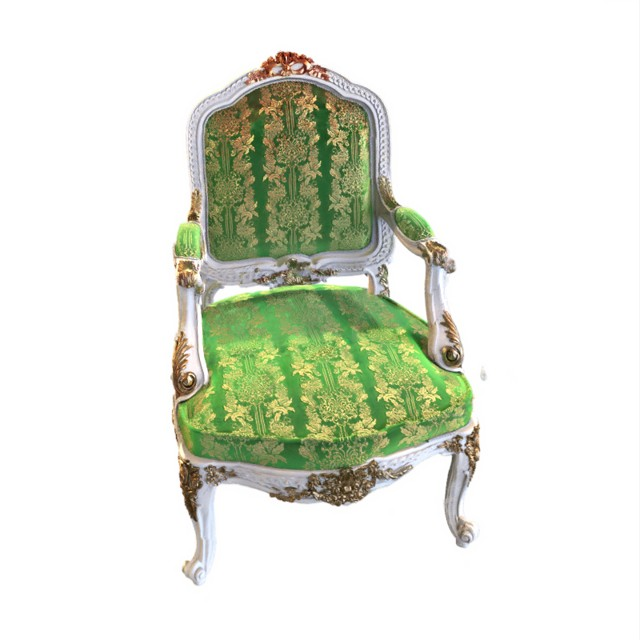}}
  \mpage{0.12}{\includegraphics[width=\linewidth]{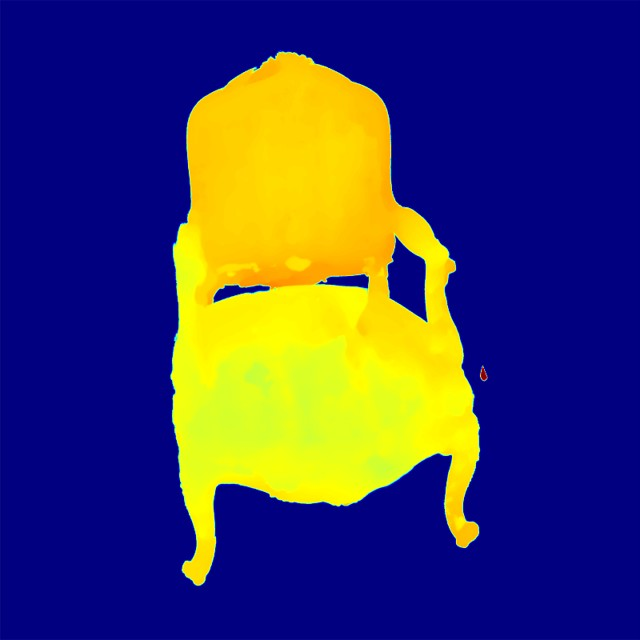}}
  \mpage{0.12}{\includegraphics[width=\linewidth]{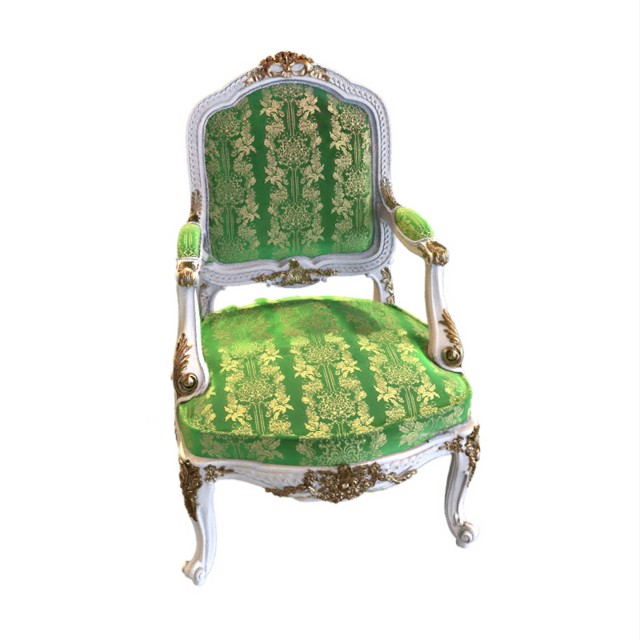}}
  \mpage{0.12}{\includegraphics[width=\linewidth]{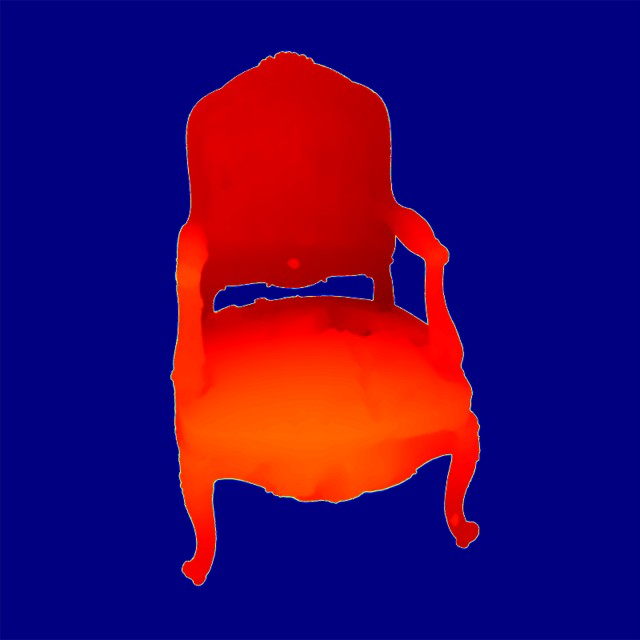}}
  \mpage{0.12}{\includegraphics[width=\linewidth]{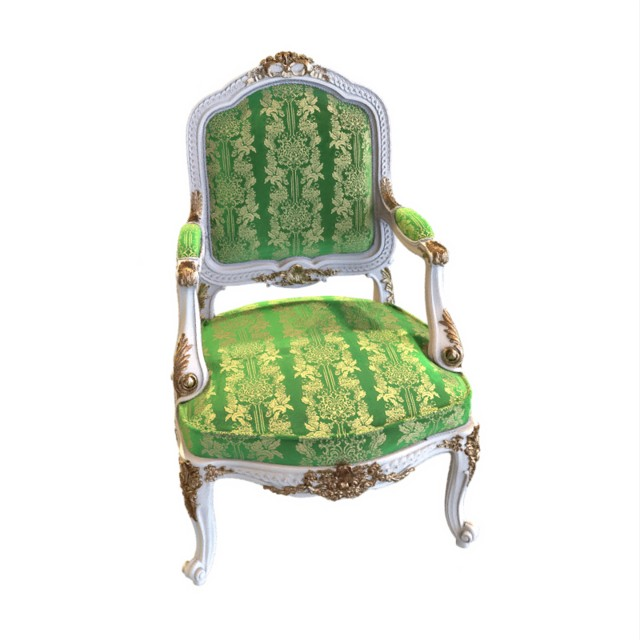}}
  \mpage{0.12}{\includegraphics[width=\linewidth]{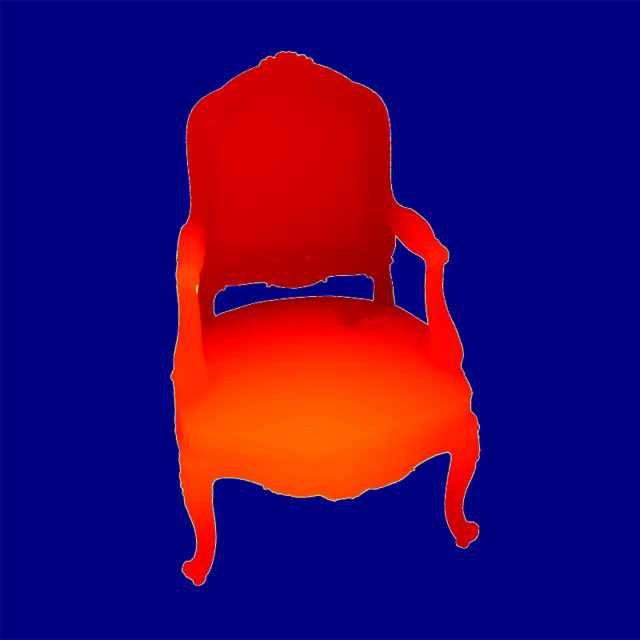}}
  \\

  \mpage{0.05}{\ }
  \mpage{0.115}{Ground Truth}
  \mpage{0.115}{ours (3)}
  \mpage{0.115}{ours (3 depth)}
  \mpage{0.115}{ours (6)}
  \mpage{0.115}{ours (6 depth)}
  \mpage{0.115}{ours (9)}
  \mpage{0.115}{ours (9 depth)}
  \caption{}
  \label{fig:nvs}
\end{figure}
